# Supplementary material for: Informed Steiner Trees: Sampling and Pruning for Multi-Goal Path Finding in High Dimensions
Source: arXiv:2205.04548 source file (2022-05-09)
Supplement: Supplementary file 1 [file 007-appendix.tex]

\section{Appendix}

\subsection{More Details on the Prior Work}

%While the problem of shortest path for single source and destination with motion planning has received widespread attention in the literature, the MGPF problem in continuous domains also referred to as multi-goal motion planning) has not been studied as extensively. In this section, we provide a review of the existing work for MGPF in continuous domains and its related variants. 

% Additionally, dynamics \cite{edelkamp2014multi, edelkamp2017surface, faigl2019fast}, energy constraints \cite{warsame2020energy}, and range constraints \cite{mcmahon2021dynamic} have also been considered in relation to Multi-goal path-finding, which our work does not consider. However with additional effort our work can be extended to incorporate such aspects.
%However, there have been works considering it in varying extent which we address below. 

Self-organizing maps (SOM) have been used to solve MGPF \cite{fort1988solving, faigl2011application}. SOM is a two-layer neural network and is a iterative procedure that provides a nonlinear mapping between a higher dimensional space (set of goals) to a lower dimensional one (goal ordering). SOM also relies on an underlying distance metric, which can be Euclidean \cite{fort1988solving}, visibility graph-based \cite{faigl2011application,faigl2013visiting}, or sampling-based graph approximation \cite{faigl2016self, vanvek2014multi}. However, in comparison to our asymptotic 2-approximation guarantee, there is no guarantee on the quality of solutions obtained using SOMs. 
 
In {\cite{faigl2011application,faigl2013visiting}, a point robot moves in an environment represented as a polygonal domain, and a convex polygon partition is used for workspace decomposition. Such assumptions may not be straightforward to generalize, for example, such a decomposition is not possible even in common robotic environments like SE(3); thus, making them incomparable to {\alg IST\textsuperscript{*}} in the environments considered.}

Multi-goal motion planning has also been explored in application to data collection. \cite{faigl2014unifying} consider this problem in planar environment with neighborhood and prize on the goals. The vehicle is required to visit only the neighborhood of each goal and all the goal (regions) are not given the same priority. This makes their problem significantly different from the one we have addressed. Similarly, \cite{mcmahon2021dynamic} have considered rewards on goals but also assume the fact that both goals and rewards are unknown to the operating vehicle in the beginning and become known only when a goal comes under its sensing radius. 

\cite{faigl2019fast} consider the generalized traveling salesman problem with neighborhoods (GTSPN) \emph{specifically for 3D environments}, where an individual neighborhood may consist of multiple regions (thus, forming a neighborhood set), and the problem is to determine a shortest multi-goal path to visit at least one region of each neighborhood. They propose two heuristics for solving the GTSPN with neighborhoods defined as polyhedra and ellipsoids to quickly find a feasible solution. The heuristics exploit properties of the 3D instances with convex regions making their approach inapplicable for comparison with ours. Further, they mention that an extension of their proposed approach for high-dimensional problems is a subject of their future work, which precisely forms the motivation for our work. 

Other papers have addressed variations of multi-goal motion planning taking into account additional constraints like Dubins vehicle \citep{faigl2020fast}, energy-aware planning with recharging stations \citep{warsame2020energy}, availability of physics-based game engine to model dynamics \citep{edelkamp2014multi} which are outside our scope. 

There is also an extensive literature on efficiently constructing minimal-cost Euclidean Steiner Tree spanning a set of vertices on a plane avoiding obstacles, having applications in VLSI designs and ascent assembly engineering \cite{zuavoianu2018multi, lin2008obstacle, decroos2015solving}. However, they assume the underlying (roadmap) graph whose nodes act as Steiner points to be given up-front as input rather than constructing and refining it over time to reduce the path cost.

% In distantly related work, Manadalika et. al. have studied 

Finally, we would like to emphasize that the major difference in our proposed approach with respect to prior work is to adapt informed sampling (with a pruning method based on the current bounds on the edge lengths) to the setting of multiple goals enabling faster convergence to an asymptotically 2-approximate solution.

%\section{Incremental MPGF}

\subsection{Key Lemma on Ripple}
We will prove Lemma 2 %~\ref{lem:voronoi} 
here by induction.
At the beginning of the algorithm, $G$ consists only of the terminals $t' \in T$ for which $r_{t'} = t'$ so the claim is trivially true.
When a new sample point $s$ is processed, it is assigned to its neighbor $n$ with the smallest value of $g(n) + cost(s,n)$ (line 6 of Algorithm 3) via which it traces a shortest path to its closest terminal (by the definition of the $g$-values of its neighbors).
The subsequent ripple of updates via the priority queue update the value of $g(n)$ and the closest terminals for neighbors $n$ who have just discovered their shortest path to a terminal via the currently processed $u^*$, and they are entered into a priority queue for further expansion. In this way, if a new shorter path via the newly added sample node $s$ arises in $G$, the  {\alg Ripple} update discovers and updates this information correctly hence maintaining the inductive invariant of the lemma that $r_u$ is (one of) the closest terminals to $u$ among all terminals $T$ for every node $u \in G$.

\subsection{Connection Radius} 

The connection radius $\rho$ (used in determining the neighbors of a node) controls the sparseness of the roadmap graph ($G$). High values of $\rho$ will lead to a dense roadmap making graph-search algorithms (like  {\alg Ripple}) computationally expensive while low values will make the roadmap sparse but may also cause it to be disconnected. As the module PRM* from OMPL was used as the underlying roadmap for both {\alg IST\textsuperscript{*}} and the Baseline, it adaptively limits the connections in $G$ as the number of samples increase by decreasing the radius $\rho$ (generally done to make the minimal number of connections required to ensure asymptotic optimality), as proposed in \cite{karaman2011sampling}%[Algorithm 4]
\begin{align*}
     \rho(q) := \eta \Bigg( 2 \Big(1 + \frac{1}{d} \Big) \bigg( \frac{\lambda \big(X_f \big)}{\zeta_d} \bigg)
     \Big(\frac{\ log(q)}{q} \Big)
     \Bigg)^{\frac{1}{d}}
\end{align*}
where $q$ is the number of points sampled in $X_f$ (ie., $|V|$), $d$ is the dimension of $X$, $\eta > 1$ is a tuning parameter, and $\lambda(X_f)$ is Lebesgue measure of the obstacle-free space and $\zeta_d$ is the volume of the unit ball in the $d$-dimensional Euclidean space.

\fi%%%%%%%%%%%%%%%%%%%%%%%%%%%%%%%%%%%%%%%%%%%%%%%%

\subsection{Pruning}

\subsubsection{Lower Bound on Edges:}
A critical phase in {\alg IST\textsuperscript{*}} is pruning edges of $G_T$ which cannot be part of the MST in future. Success of this phase relies heavily on how close are the lower bounds of these edges to their optimal cost. Past research has been focused mostly on finding lower bounds for special instances of the general motion planning problem \cite{canny1987new, lumelsky1987path}. A separate line of research recently has been focused on calculating the lower bound on \textbf{the past cost obtainable from the current set of samples} %but not on the actual solution 
\cite{salzman2015asymptotically}. However, these are not lower bound on the optimal path cost but only representative of the lower bound derived from the discrete approximation of the state space. Thus, due to lack of effective worst-case lower bound on the optimal path cost for the general motion planning problem, we use the Euclidean distance between two points %configurations
in $X_f$ as the heuristic estimate.

\subsubsection{Numerical Results:} In Table \ref{tbl:pruningStatistics}, we show the impact of the pruning condition we have developed. Even though we have a very simple heuristic estimate as the lower bound, we are able to prune a significant number of edges. With more terminals, it is likely that edges in the MST of $G_T$ will be a straight-segments in $X_f$ (hence, the optimal path is quite close to Euclidean distance). This is turn should lead to more pruning which we observe as a trend in Table \ref{tbl:pruningStatistics}.

% Pruning Results 
\begin{table}[hbt!]
\caption{Average percentage of edges pruned from $G_T$ by {\alg IST\textsuperscript{*}} in each problem instance across 50 runs.}
\[\begin{array}{|c|c|c|c|}
\hline
\tikz{\node[below left, inner sep=1pt] (def) {\small{Environment}};%
      \node[above right,inner sep=1pt] (abc) {Terminals};%
      \draw (def.north west|-abc.north west) -- (def.south east-|abc.south east);}
 & 10 & 30 & 50 \\
\hline
\texttt{CO}\ \ \mathbb{R}^4 & 91\% & 98\% & 98\%\\
\hline 
\texttt{CO}\ \ \mathbb{R}^8 & 64\% & 84\% & 90\% \\
\hline 
\texttt{UH}\ \ \mathbb{R}^4 & 92\% & 97\% & 98\%\\
\hline 
\texttt{UH}\ \ \mathbb{R}^8 & 37\% & 79\% & 81\%\\
\hline 
HOME & 87\% & 91\% & 98\%\\
\hline 
ABSTRACT & 97\% & 98\% & 99\% \\
\hline 
\end{array}\]
\label{tbl:pruningStatistics}
\end{table}

While the pruning statistics may look appealing, it is possible to generate instances where no edges would be pruned. 

\paragraph{Worst Case:} 
Consider a problem instance with a star-shaped obstacle in the center with terminals at the concave openings between two sharp ends of the star obstacle. Further, the placement of terminals and the concave openings should be such that all terminals are near to each other while the optimal path is long and convoluted. For example, in Figure \ref{fig:WorstCaseStarProblem}, lower bound between every edge is less than the optimal cost between any two distinct terminals which means no edge will be pruned in $G_T$. 

\begin{figure}[h]
  \centering
  \includegraphics[width=0.99\linewidth]{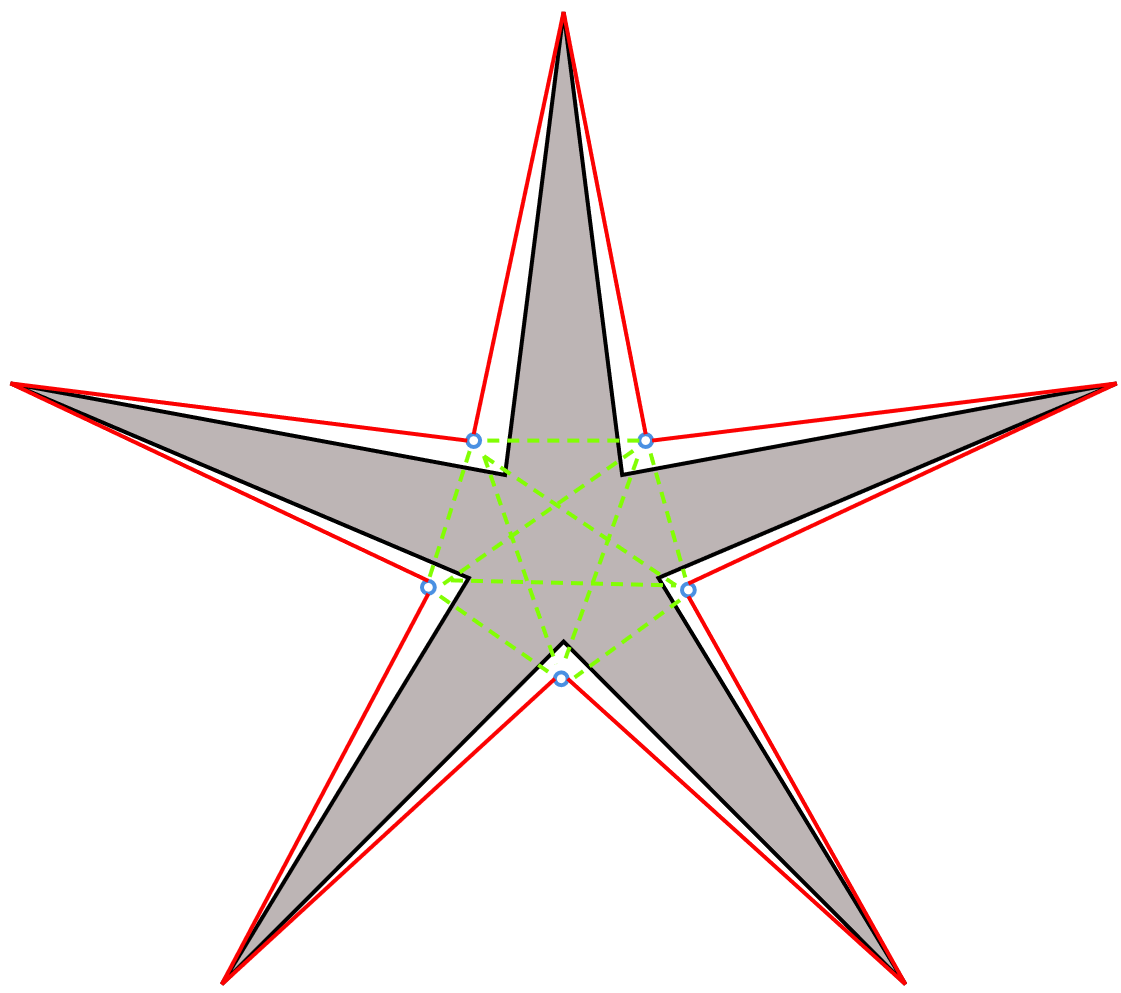}
  \caption{A problem instance: Light brown star denotes the obstacle region. Small blue hollow circles represent the terminals. The dashed green line is the Euclidean distance between the terminals while the red lines are the optimal paths.}
  \label{fig:WorstCaseStarProblem}
\end{figure}

\subsection{Implementation Details}

While we mention that a fixed number of samples is added to the roadmap in the pseudocode of {\alg IST\textsuperscript{*}}, the implementation could not exactly follow this as such an operation is not allowed in the available module for PRM*. However, OMPL does support growing the roadmap for a \emph{fixed amount of time}. Hence, we had a time-based implementation where in each iteration of {\alg IST\textsuperscript{*}}, the roadmap was grown for the same amount of time. Consequently, the number of samples added per iteration was not fixed and varied depending upon the time spent in collision-checking for each new sample point. We let {\alg IST\textsuperscript{*}} and the Baseline run for all of the provided time. 

Both the planners used the implementation of PRM* from OMPL  (with default parameters).We also tried LazyPRM* from OMPL but it performed worse than PRM*, contrary to our expectations. However, our approach (subsequently, the codebase of {\alg IST\textsuperscript{*}}) is modular such that LazyPRM* or any other implementation of the underlying roadmap can be used to interface with our planner.

\subsection{Ripple : More Results and Discussion}

We show the comparison of  {\alg Ripple} with S* on more environments in Table \ref{tbl:RippleAppendix}. In $Abstract$ with 10 terminals, we see  {\alg Ripple} performing better throughout while in all other instances its performance is almost same as Baseline. In real-vector space instances, it was observed that size of the roadmap in the end was much smaller compared to instances like $Home$ or $Abstract$. As the size of roadmap was tiny, so we couldn't witness the benefits of  {\alg Ripple}. We believe this was a consequence of our implementation in Python. 

Real environments like \texttt{CO} and \texttt{HR} (Fig. 2%\ref{fig:obstacleMap}
) were custom defined in Python so when the roadmap was grown for both {\alg IST\textsuperscript{*}} and the Baseline, OMPL's planners in C++ had to interface with the collision checker of these environments in Python for each point sampled in the configuration space. This made the growth of PRM in these instances extremely slow due to the constant back and forth call between Python and C++. Thus, the size of the roadmap $G$ in these envrionments was pretty small compared to $Home$ or $Abstract$ which are defined in OMPL App itself. 
% Ripple Plots
% \iffalse 

\begin{table*}[hbt!]
        \centering
        \begin{tabular}%{cM{50mm}M{50mm}M{50mm}}
        {cM{0.3\linewidth}M{0.3\linewidth}M{0.3\linewidth}}
           \toprule
            \emph{Env.} & 10 Terminals & 30 Terminals & 50 Terminals \\
            \midrule
         
   \makecell{A\\B\\S\\T\\R\\A\\C\\T} & 
  \includegraphics[width=\linewidth, height=40mm]{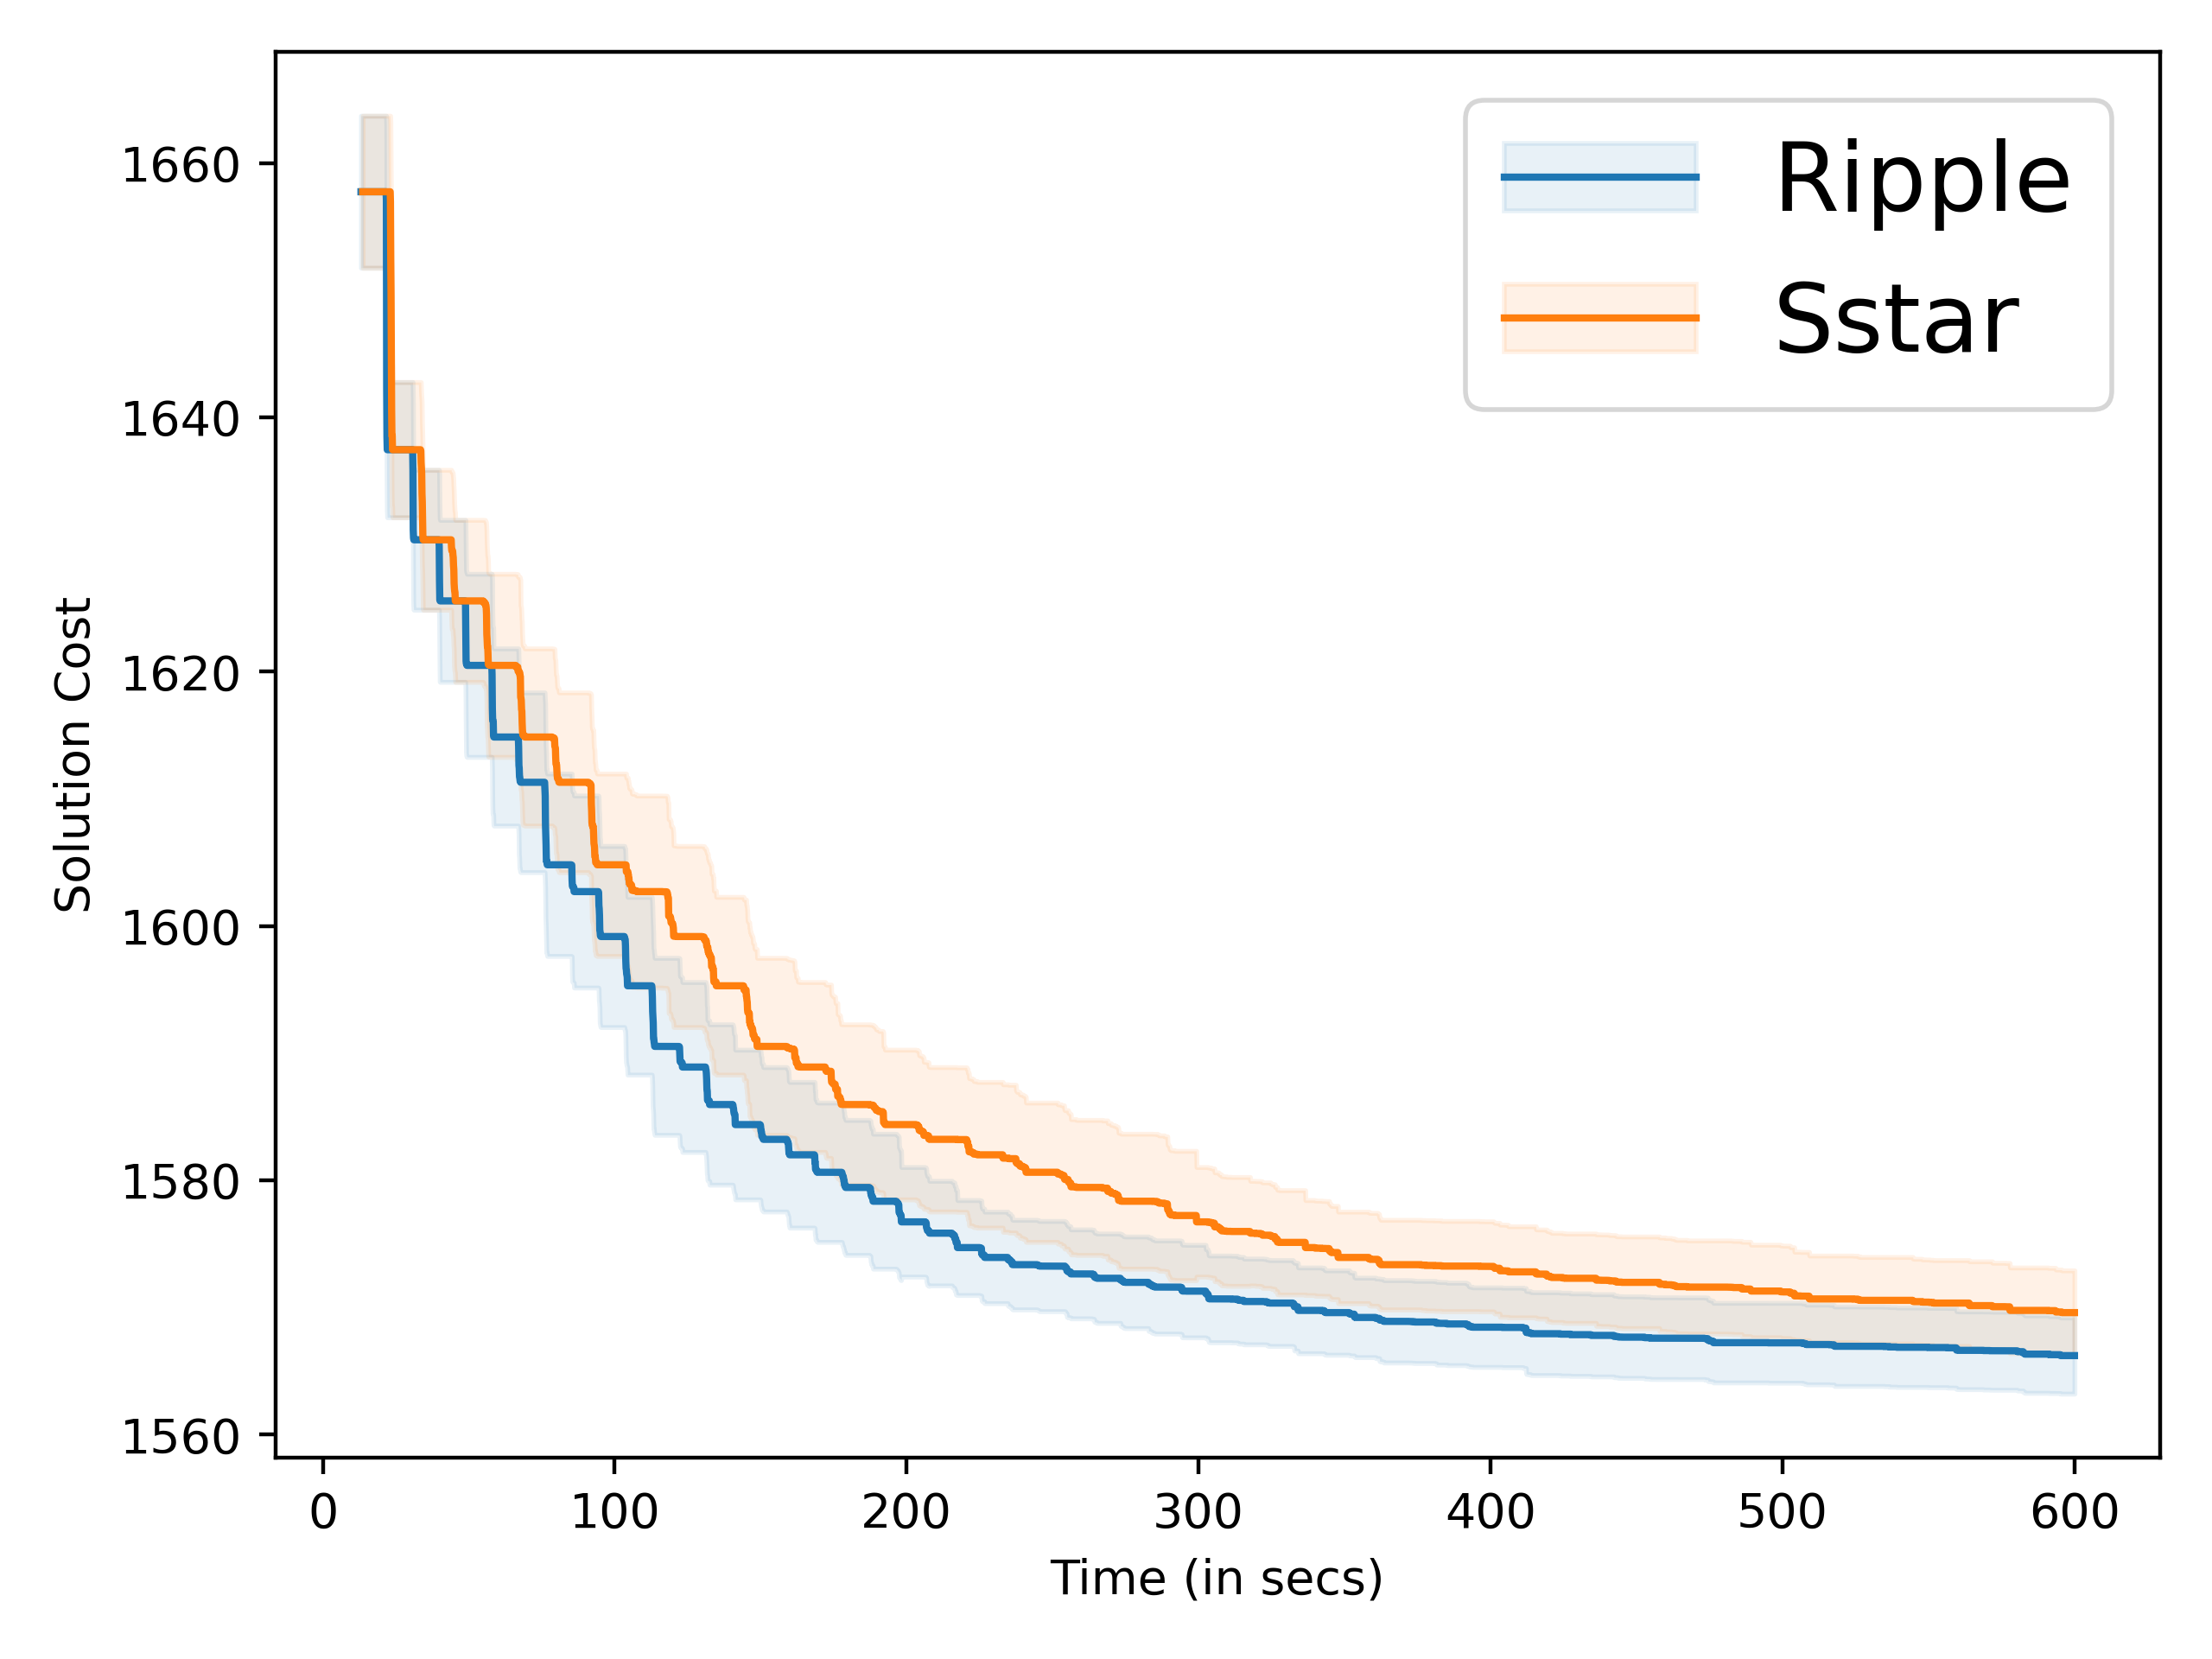}
   & \includegraphics[width=\linewidth, height=40mm]{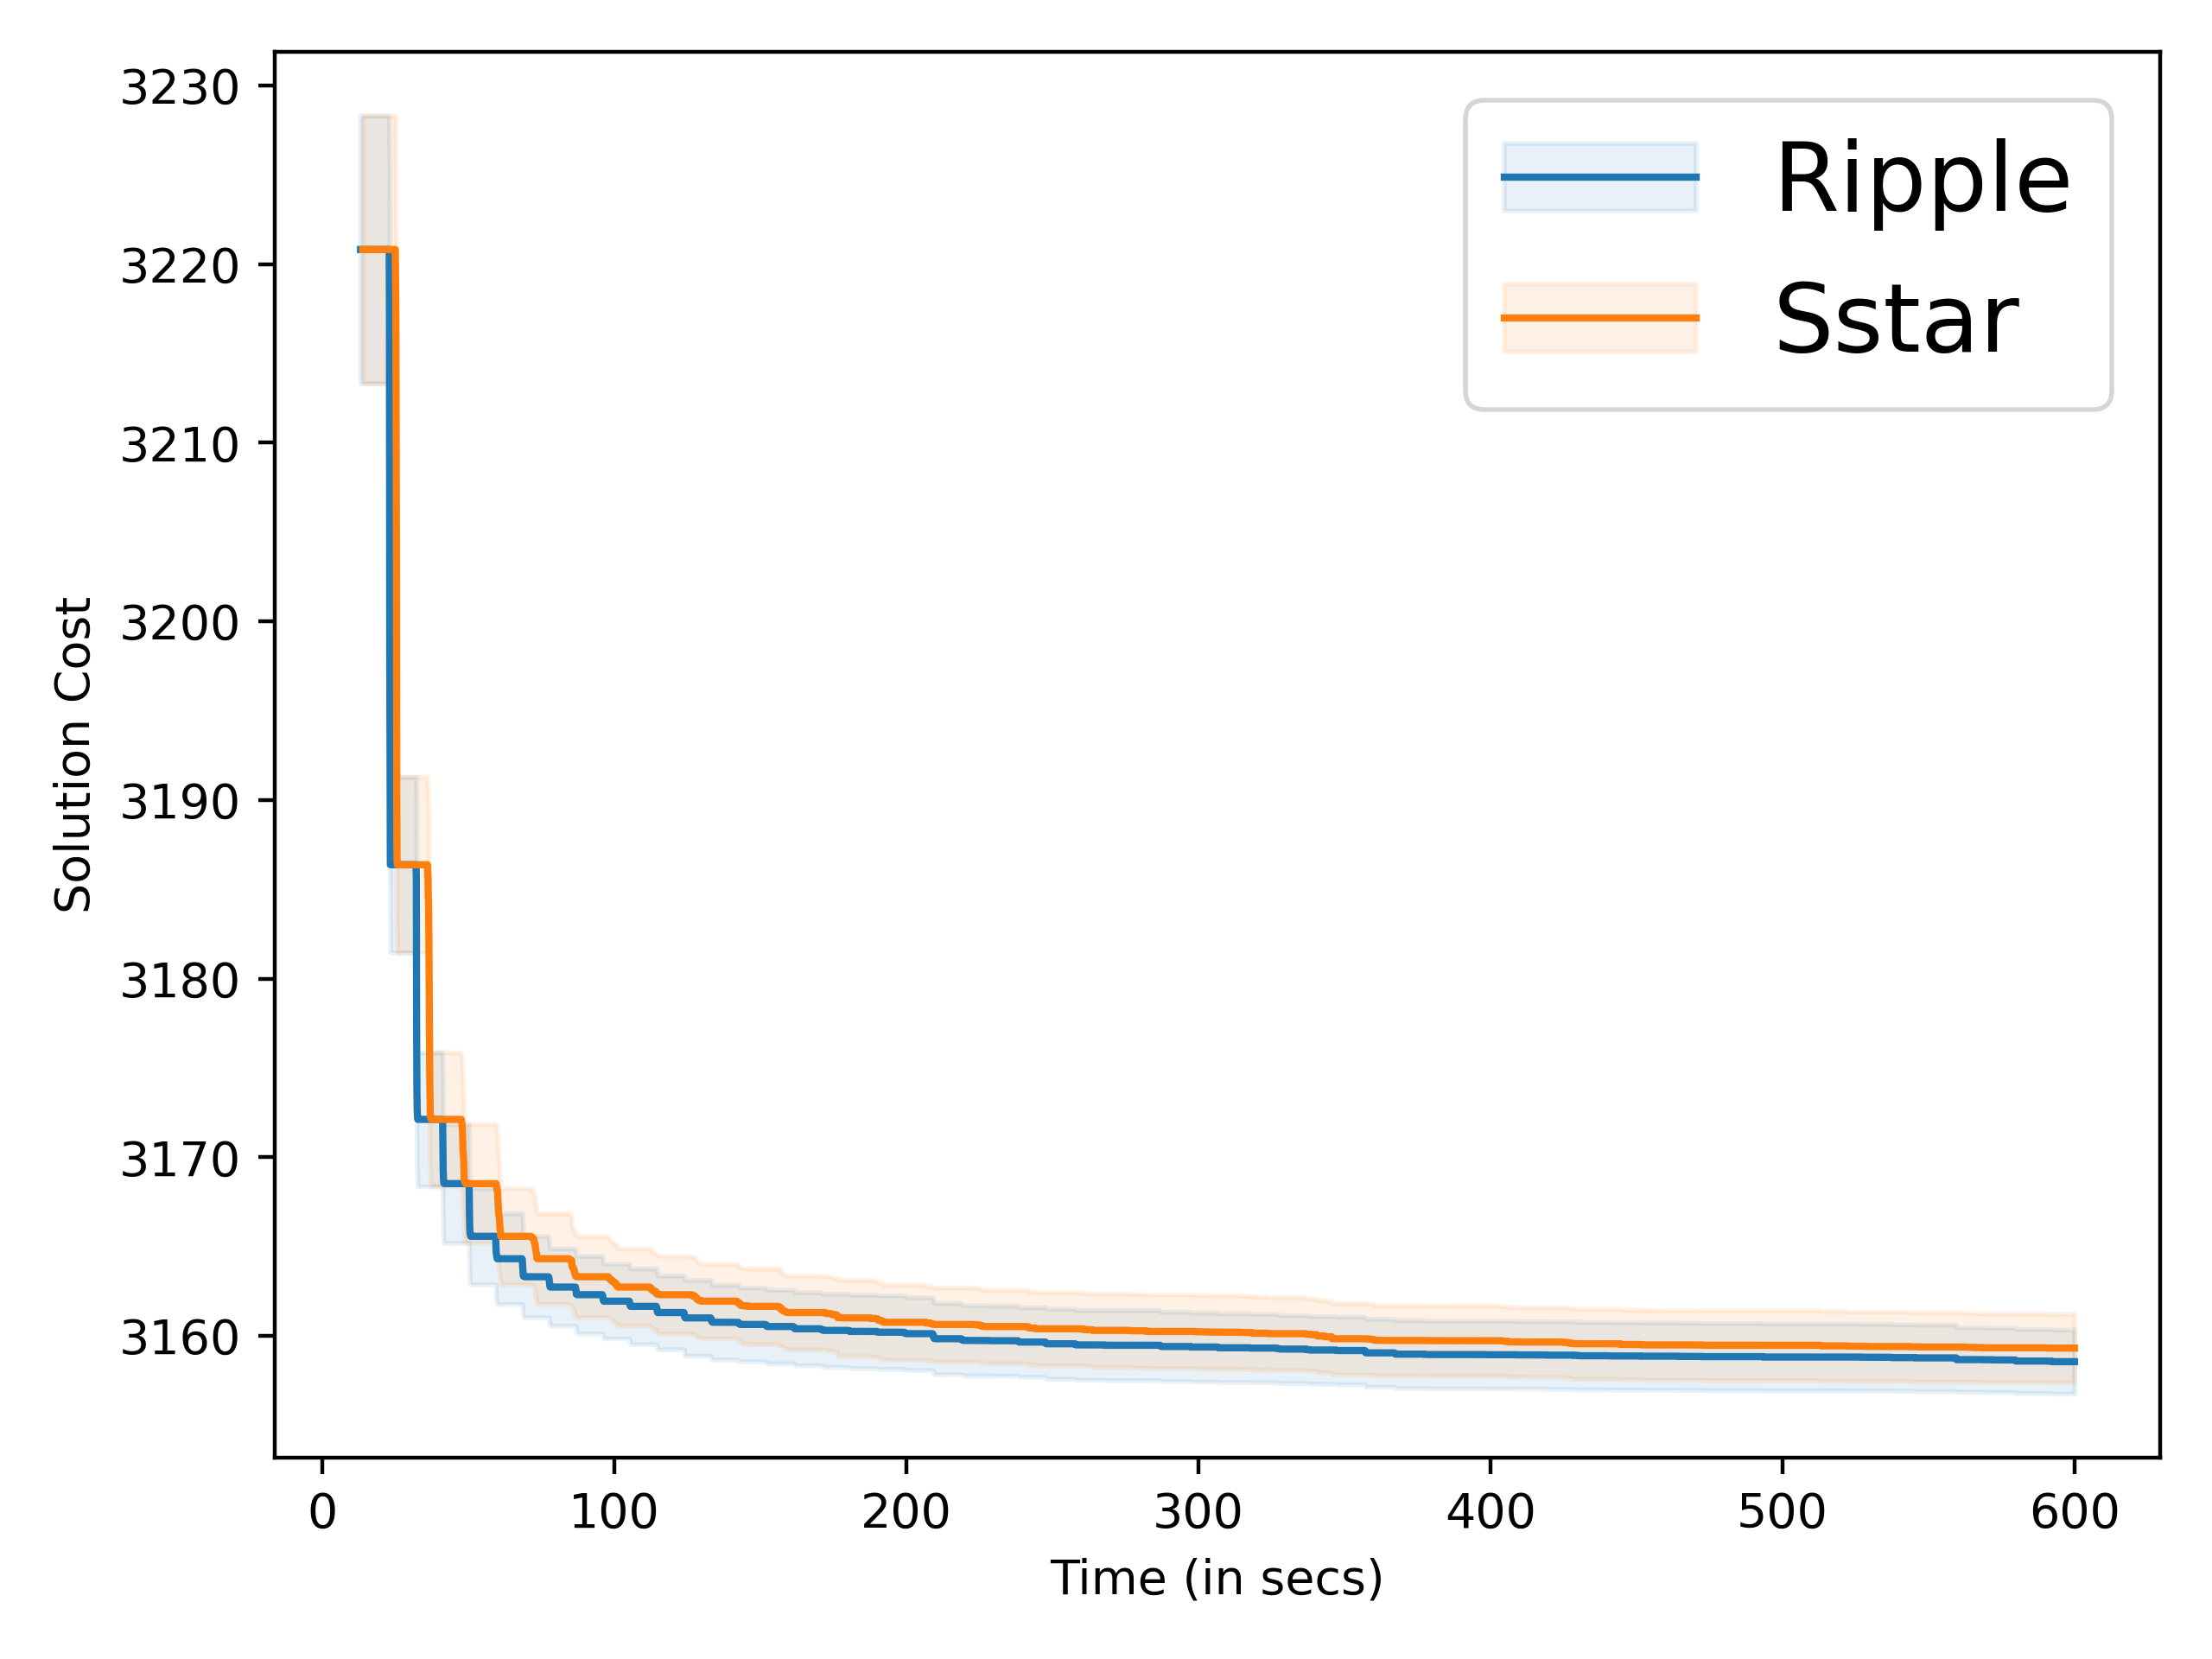} & \includegraphics[width=\linewidth, height=40mm]{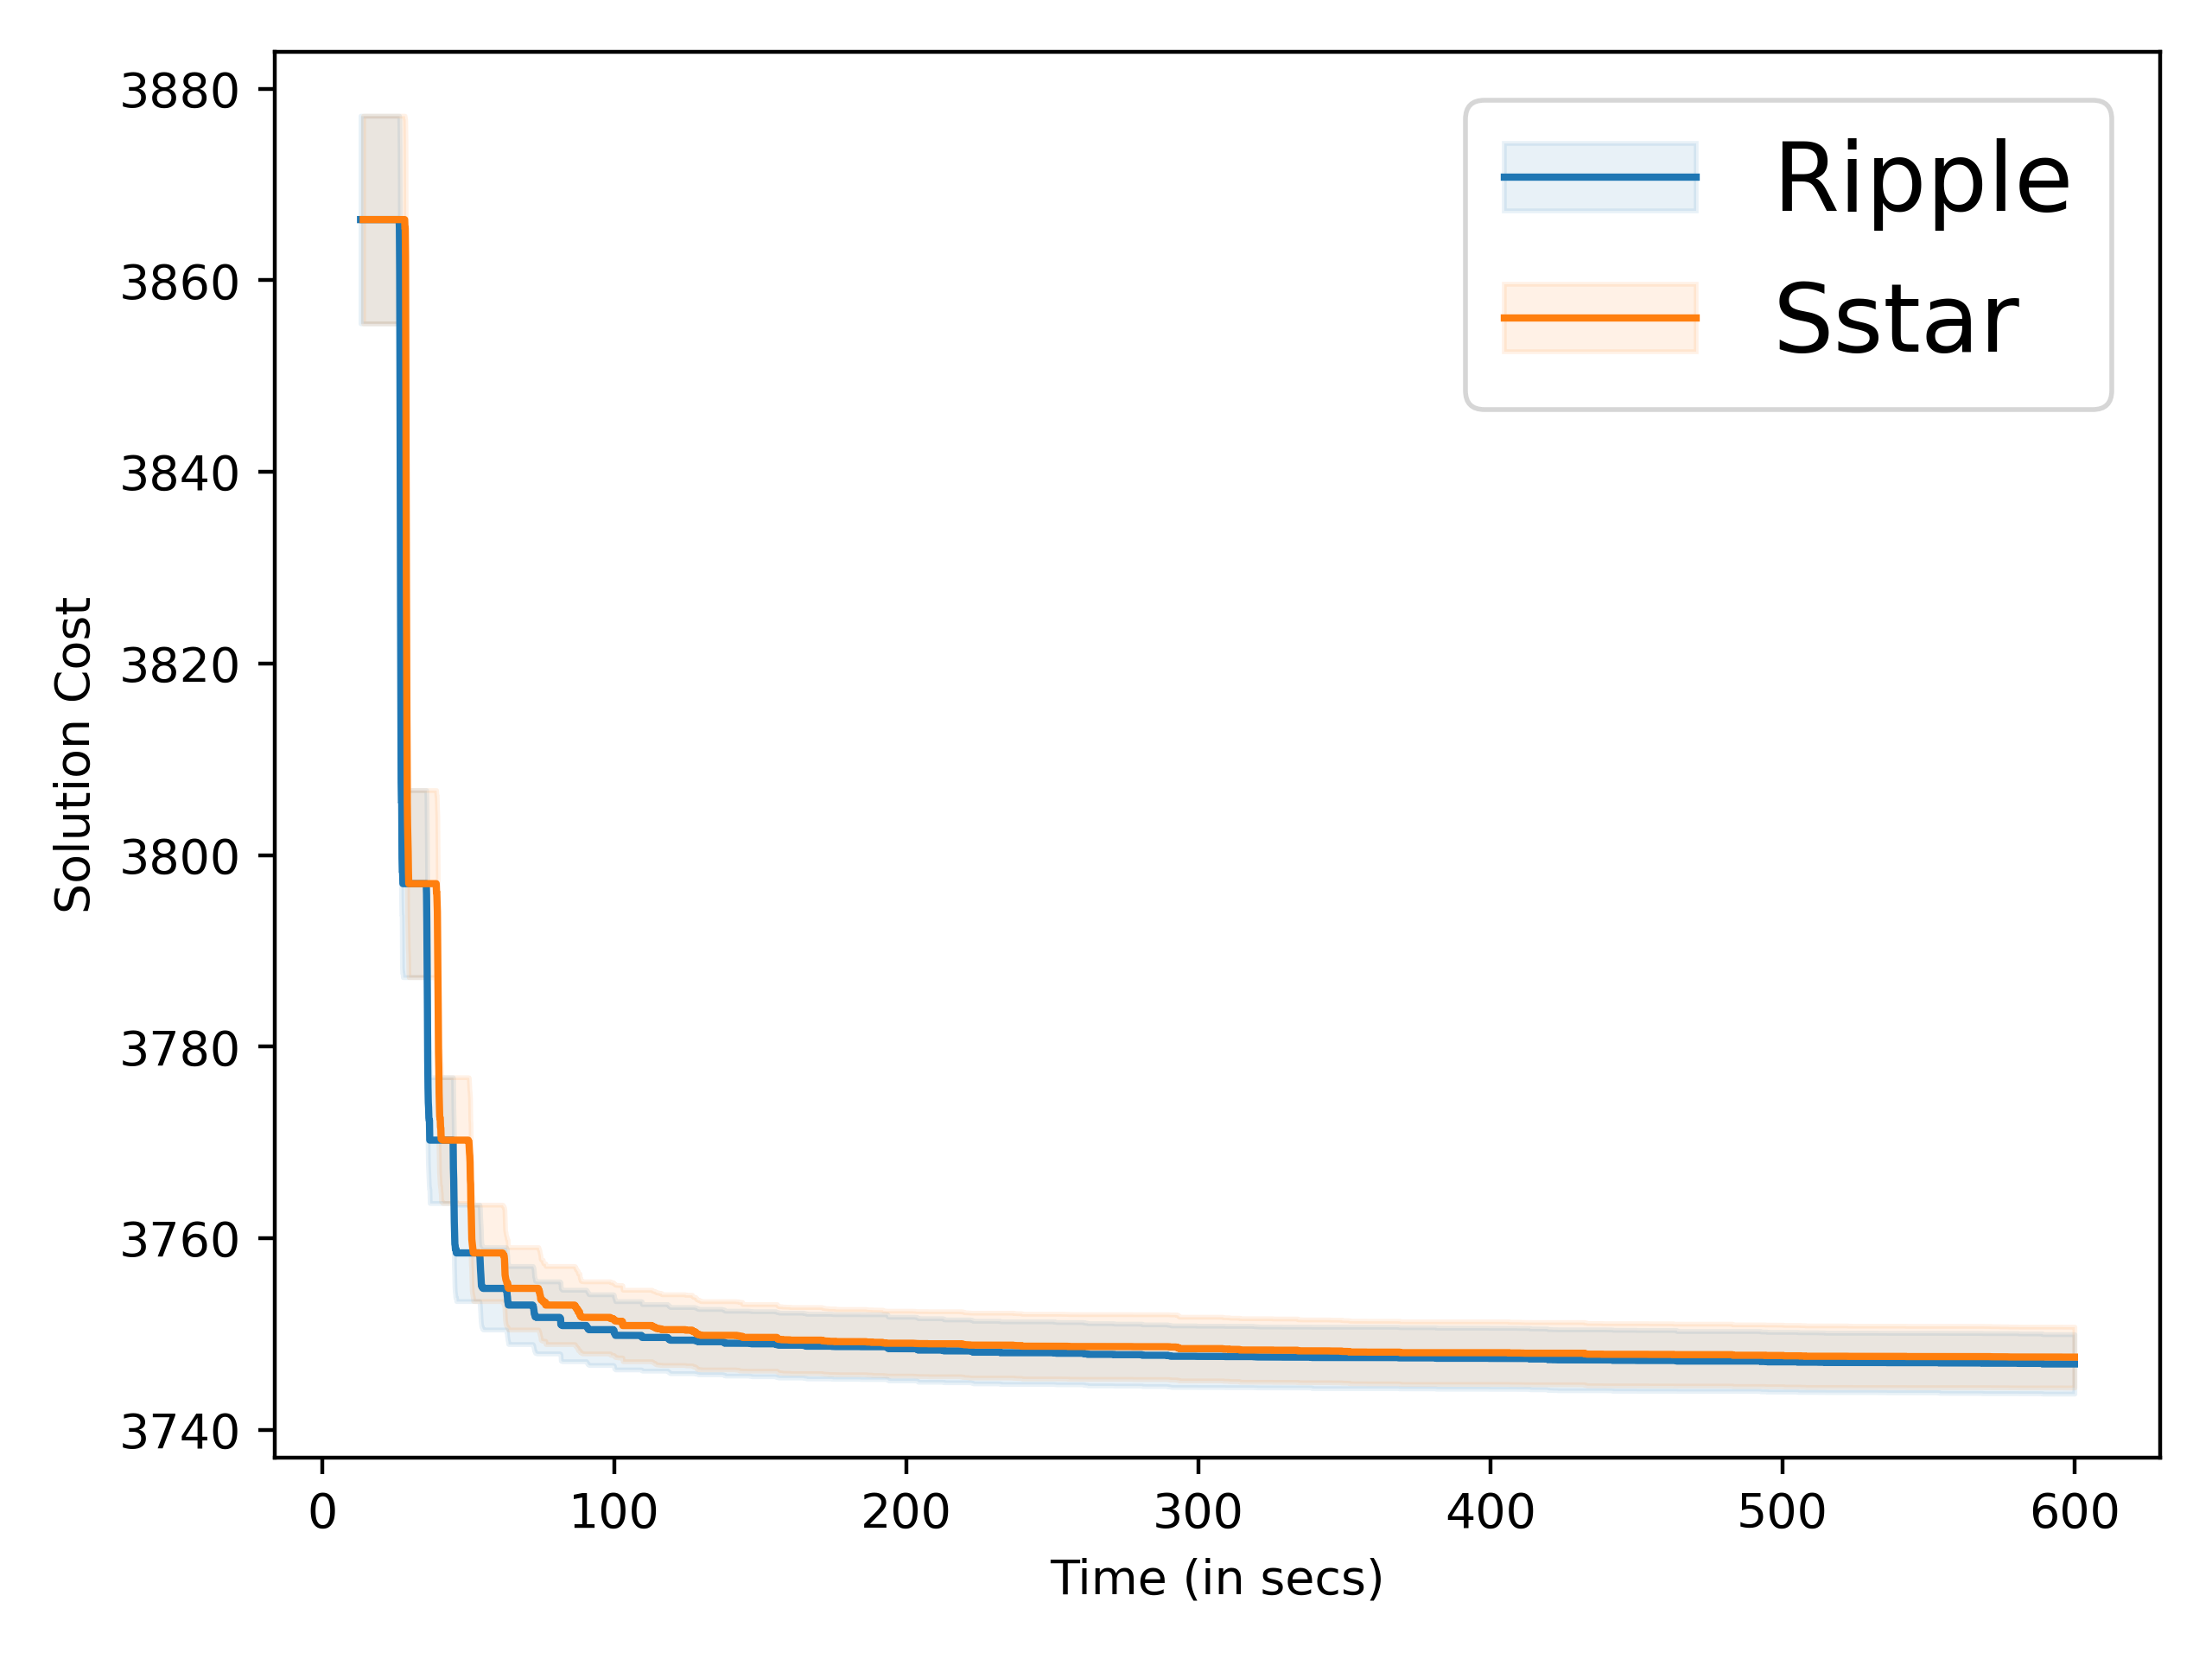} \\

   \makecell{\texttt{UH} \\ $\mathbb{R}^4$} & 
  \includegraphics[width=\linewidth, height=40mm]{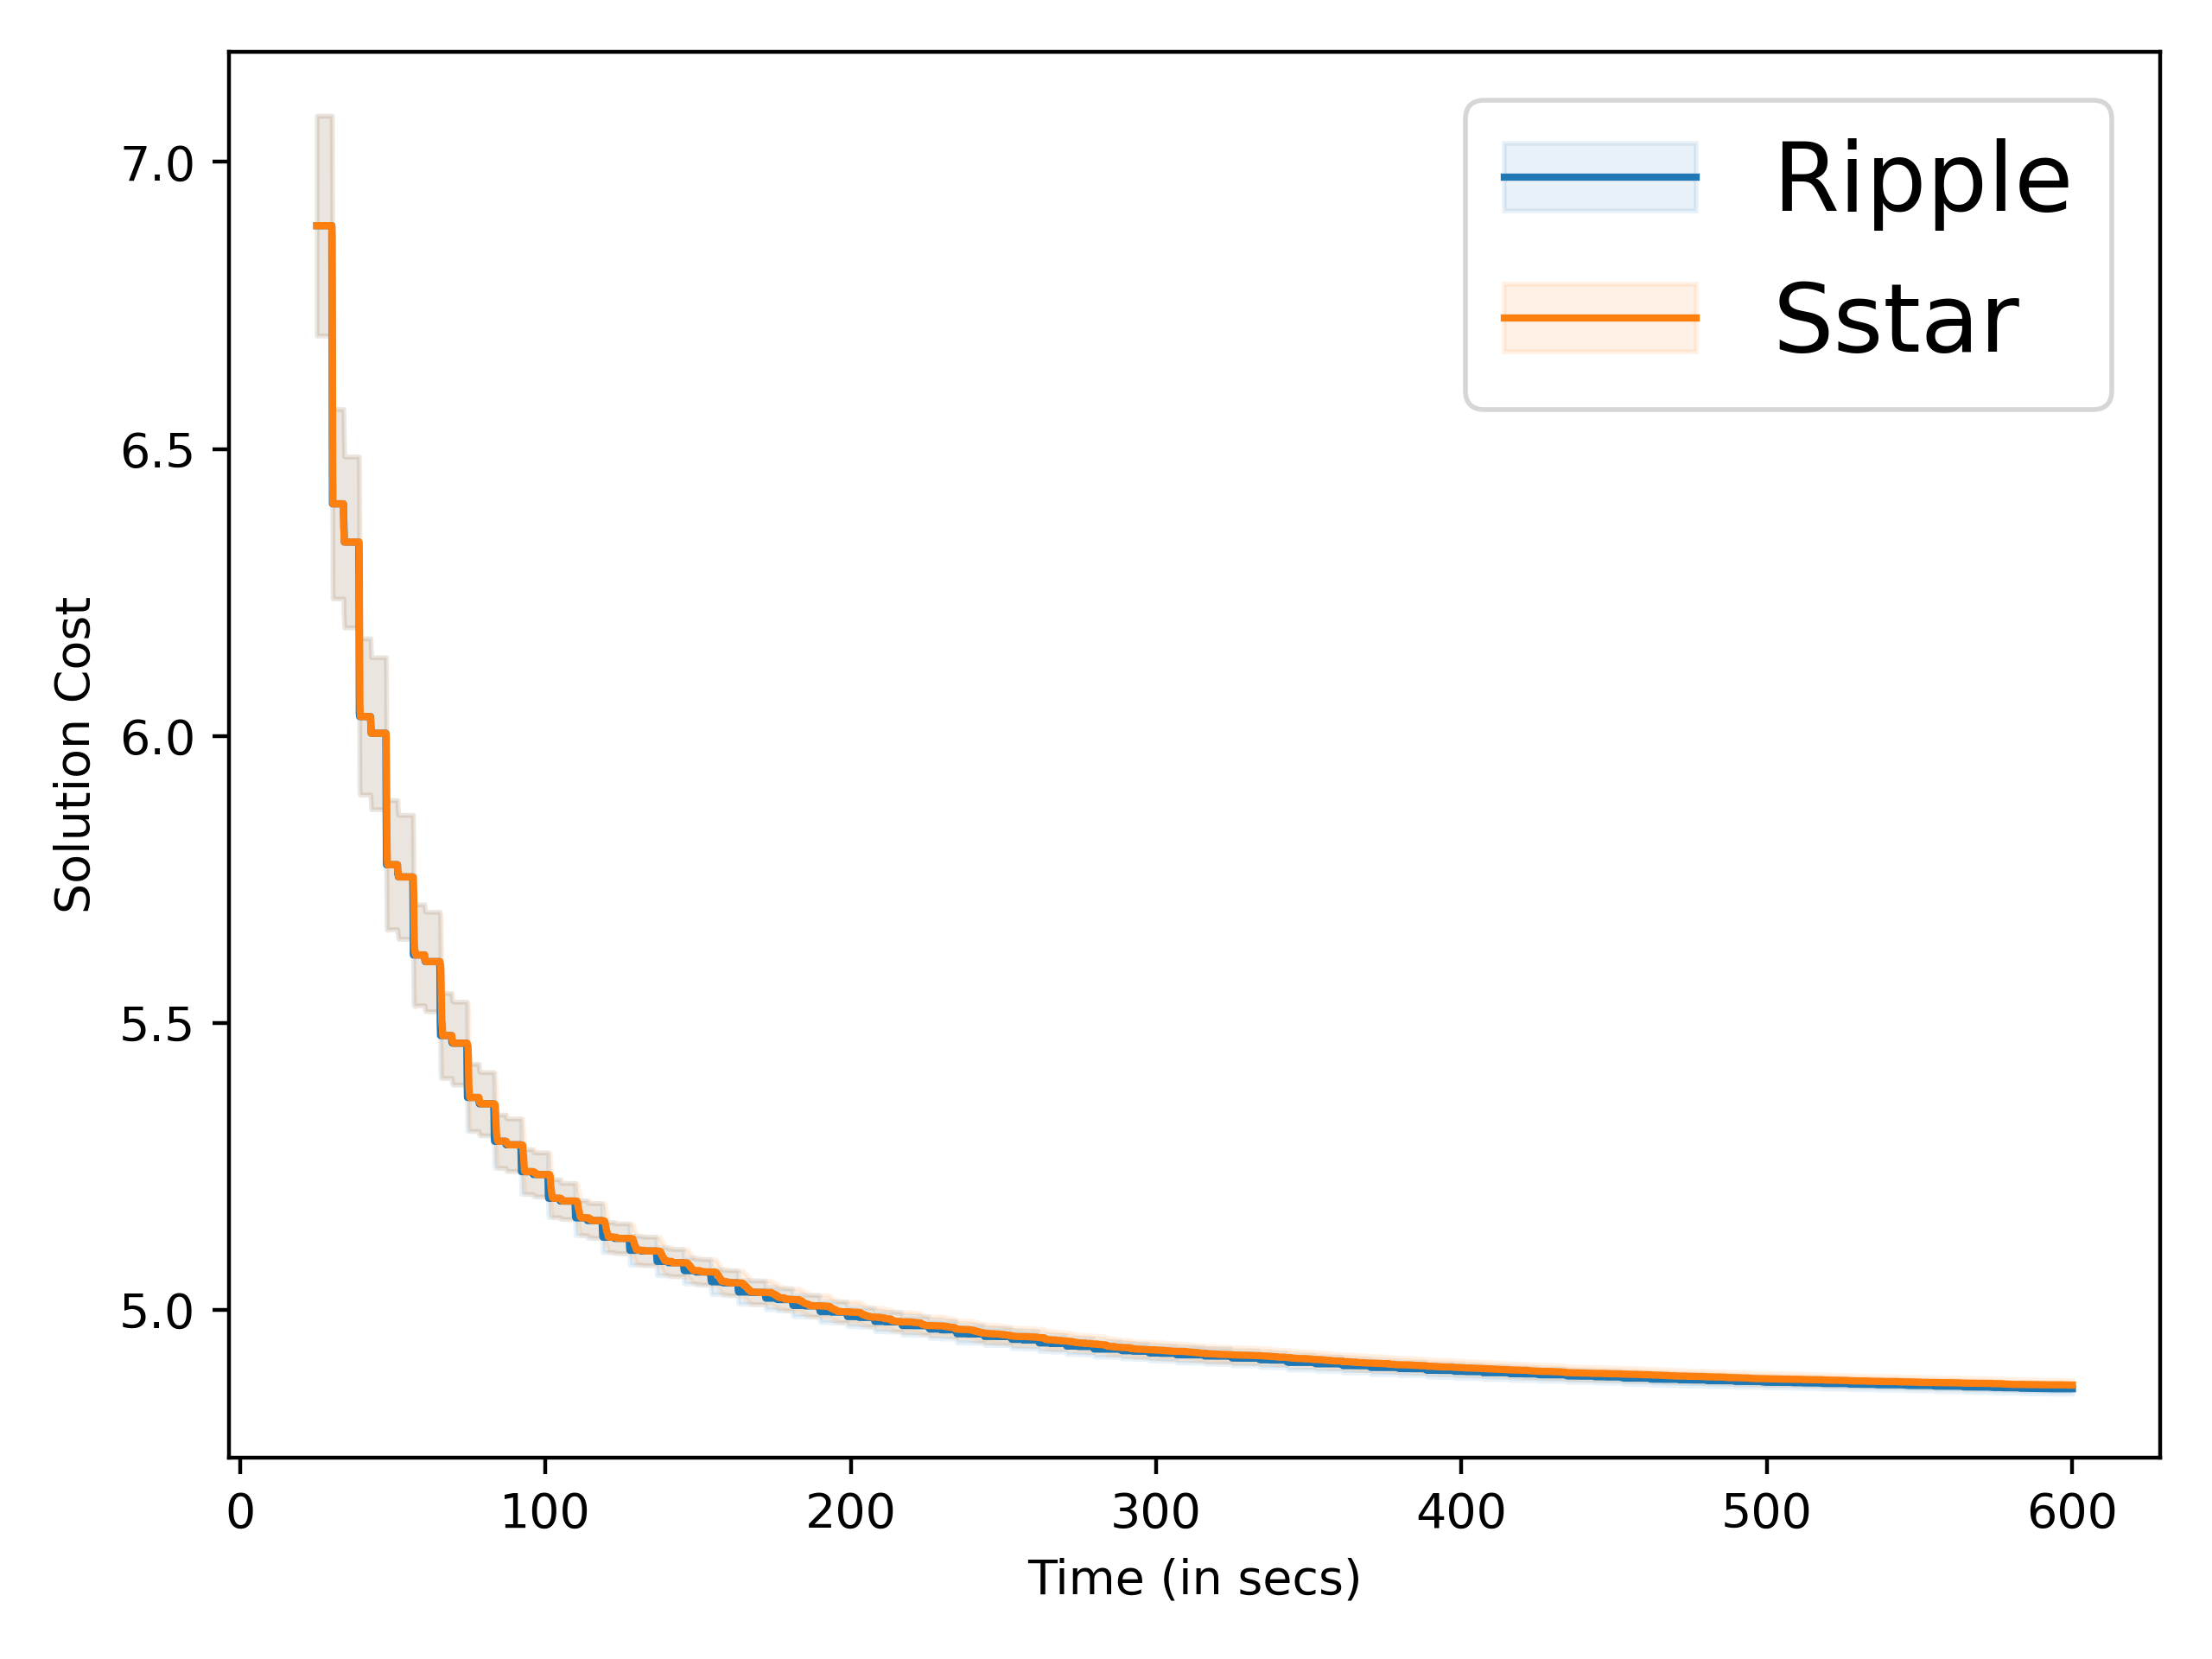}
   & \includegraphics[width=\linewidth, height=40mm]{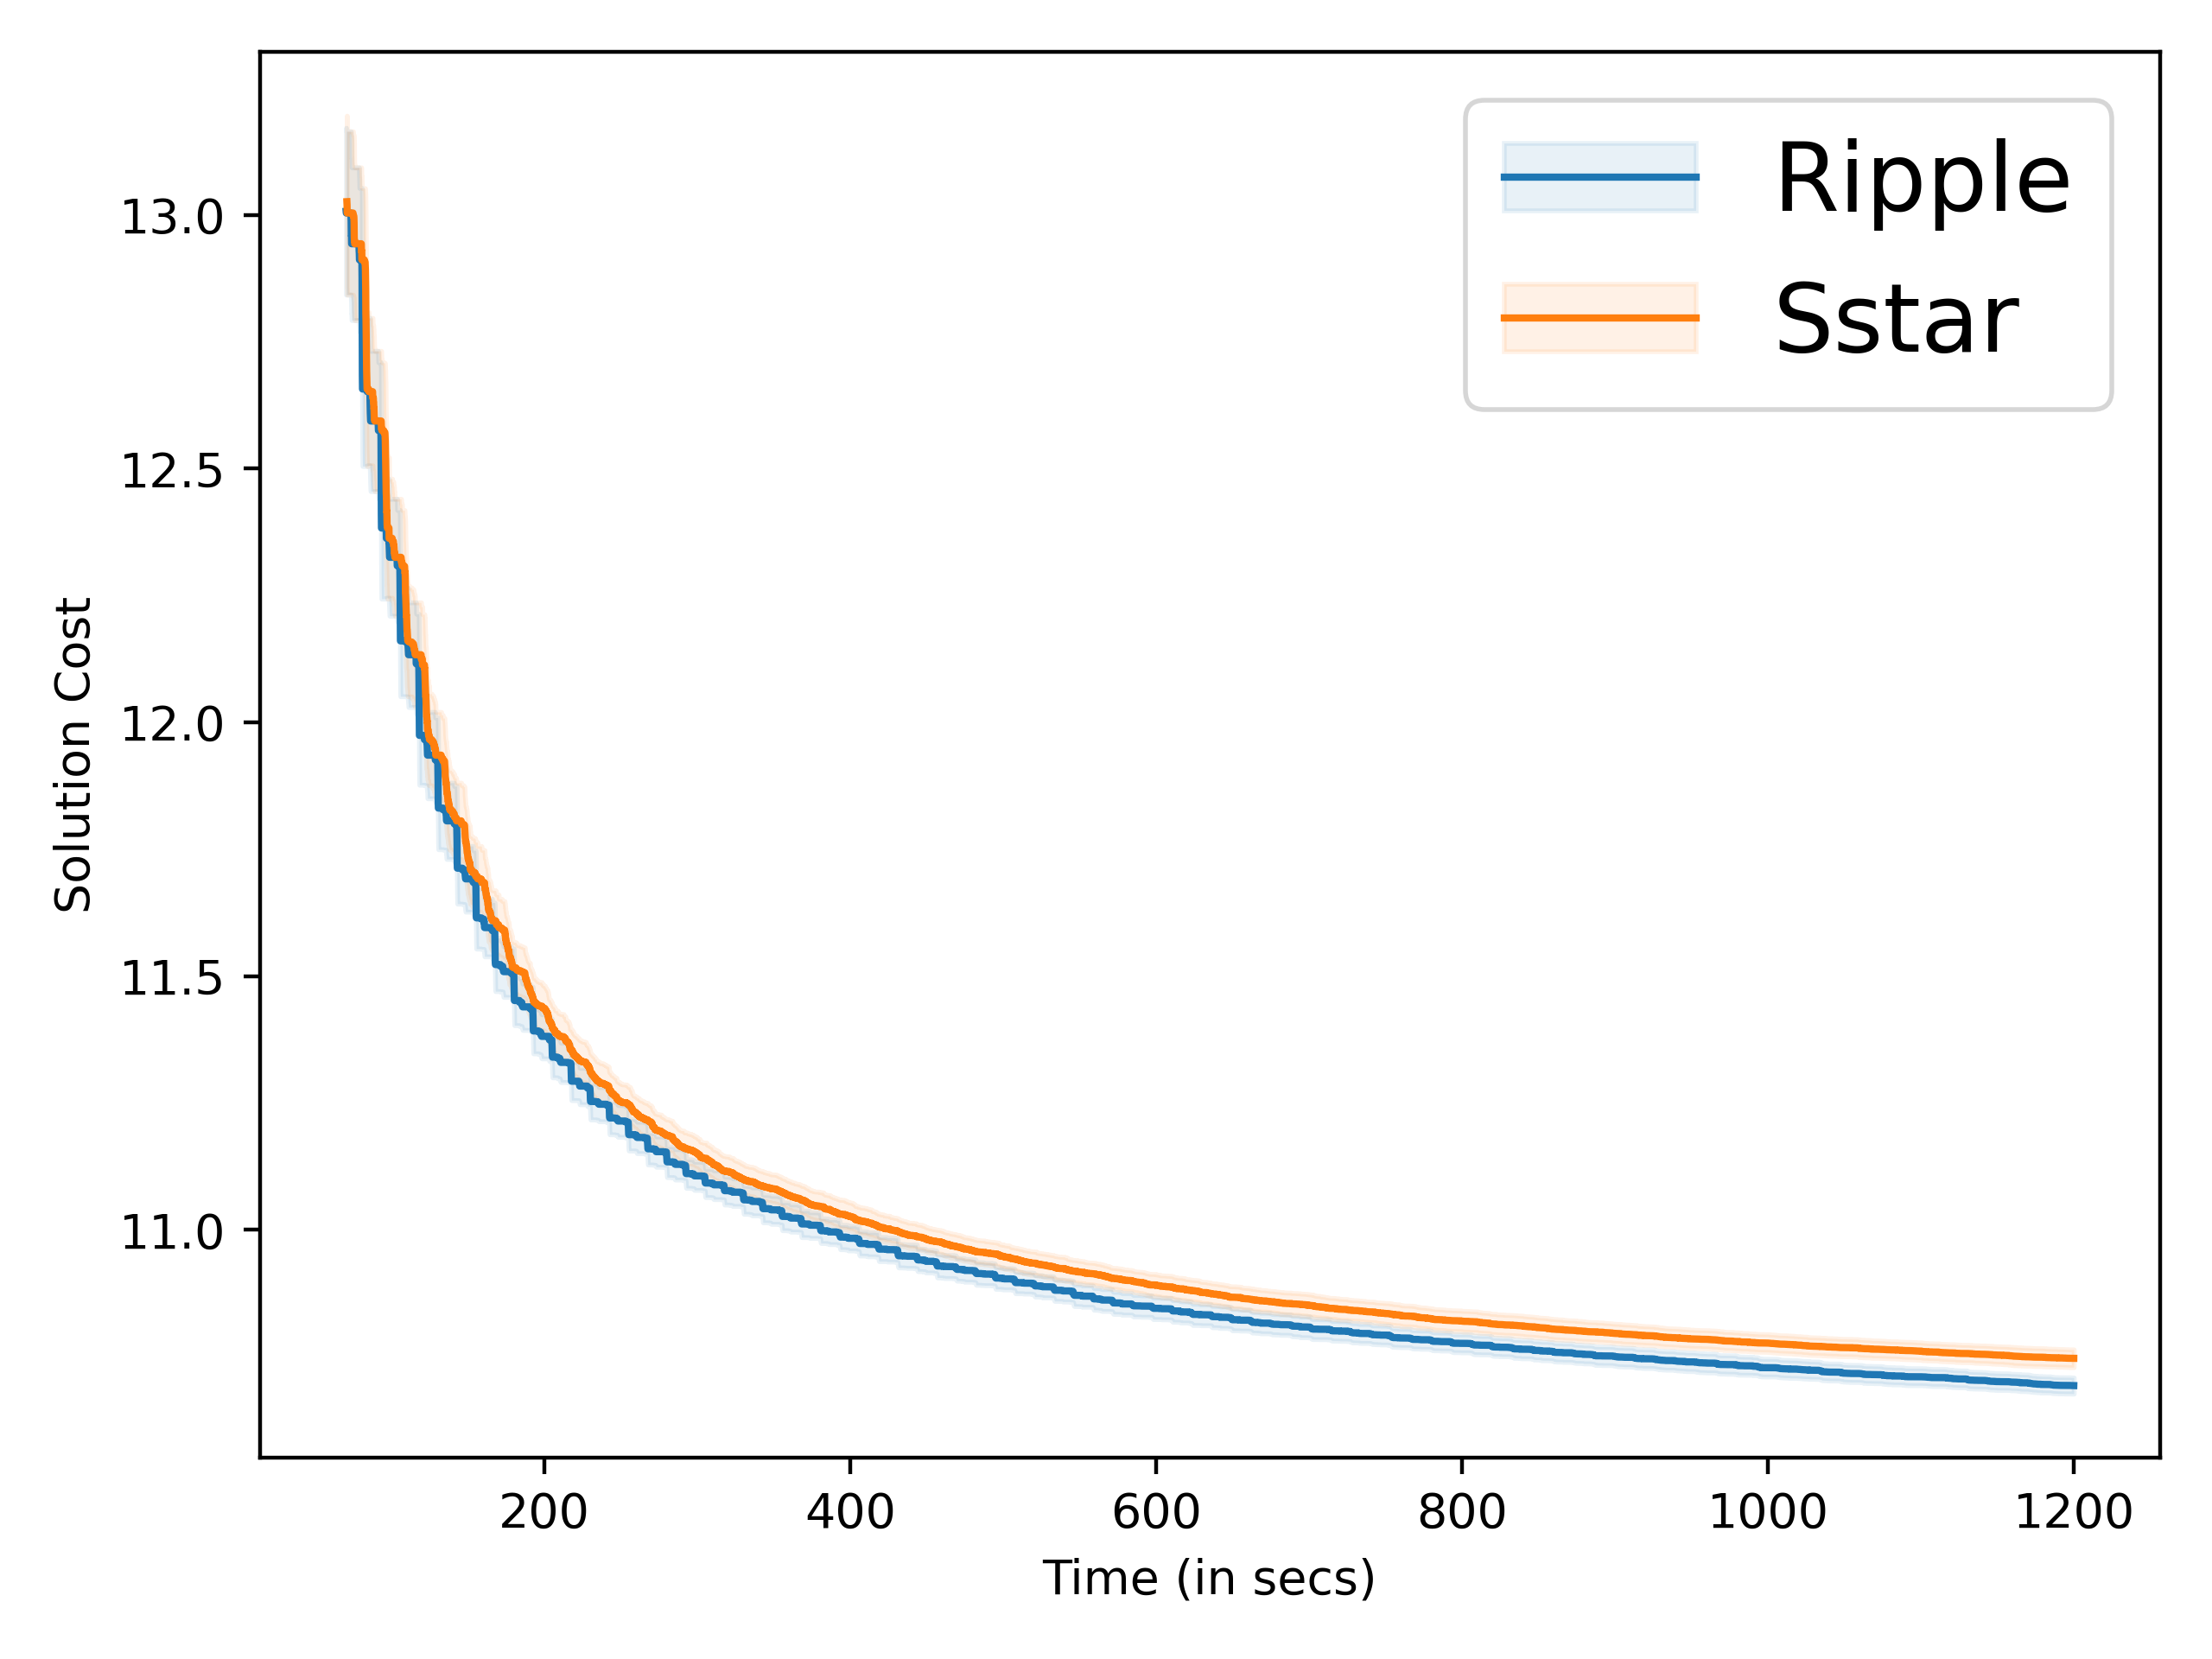} & \includegraphics[width=\linewidth, height=40mm]{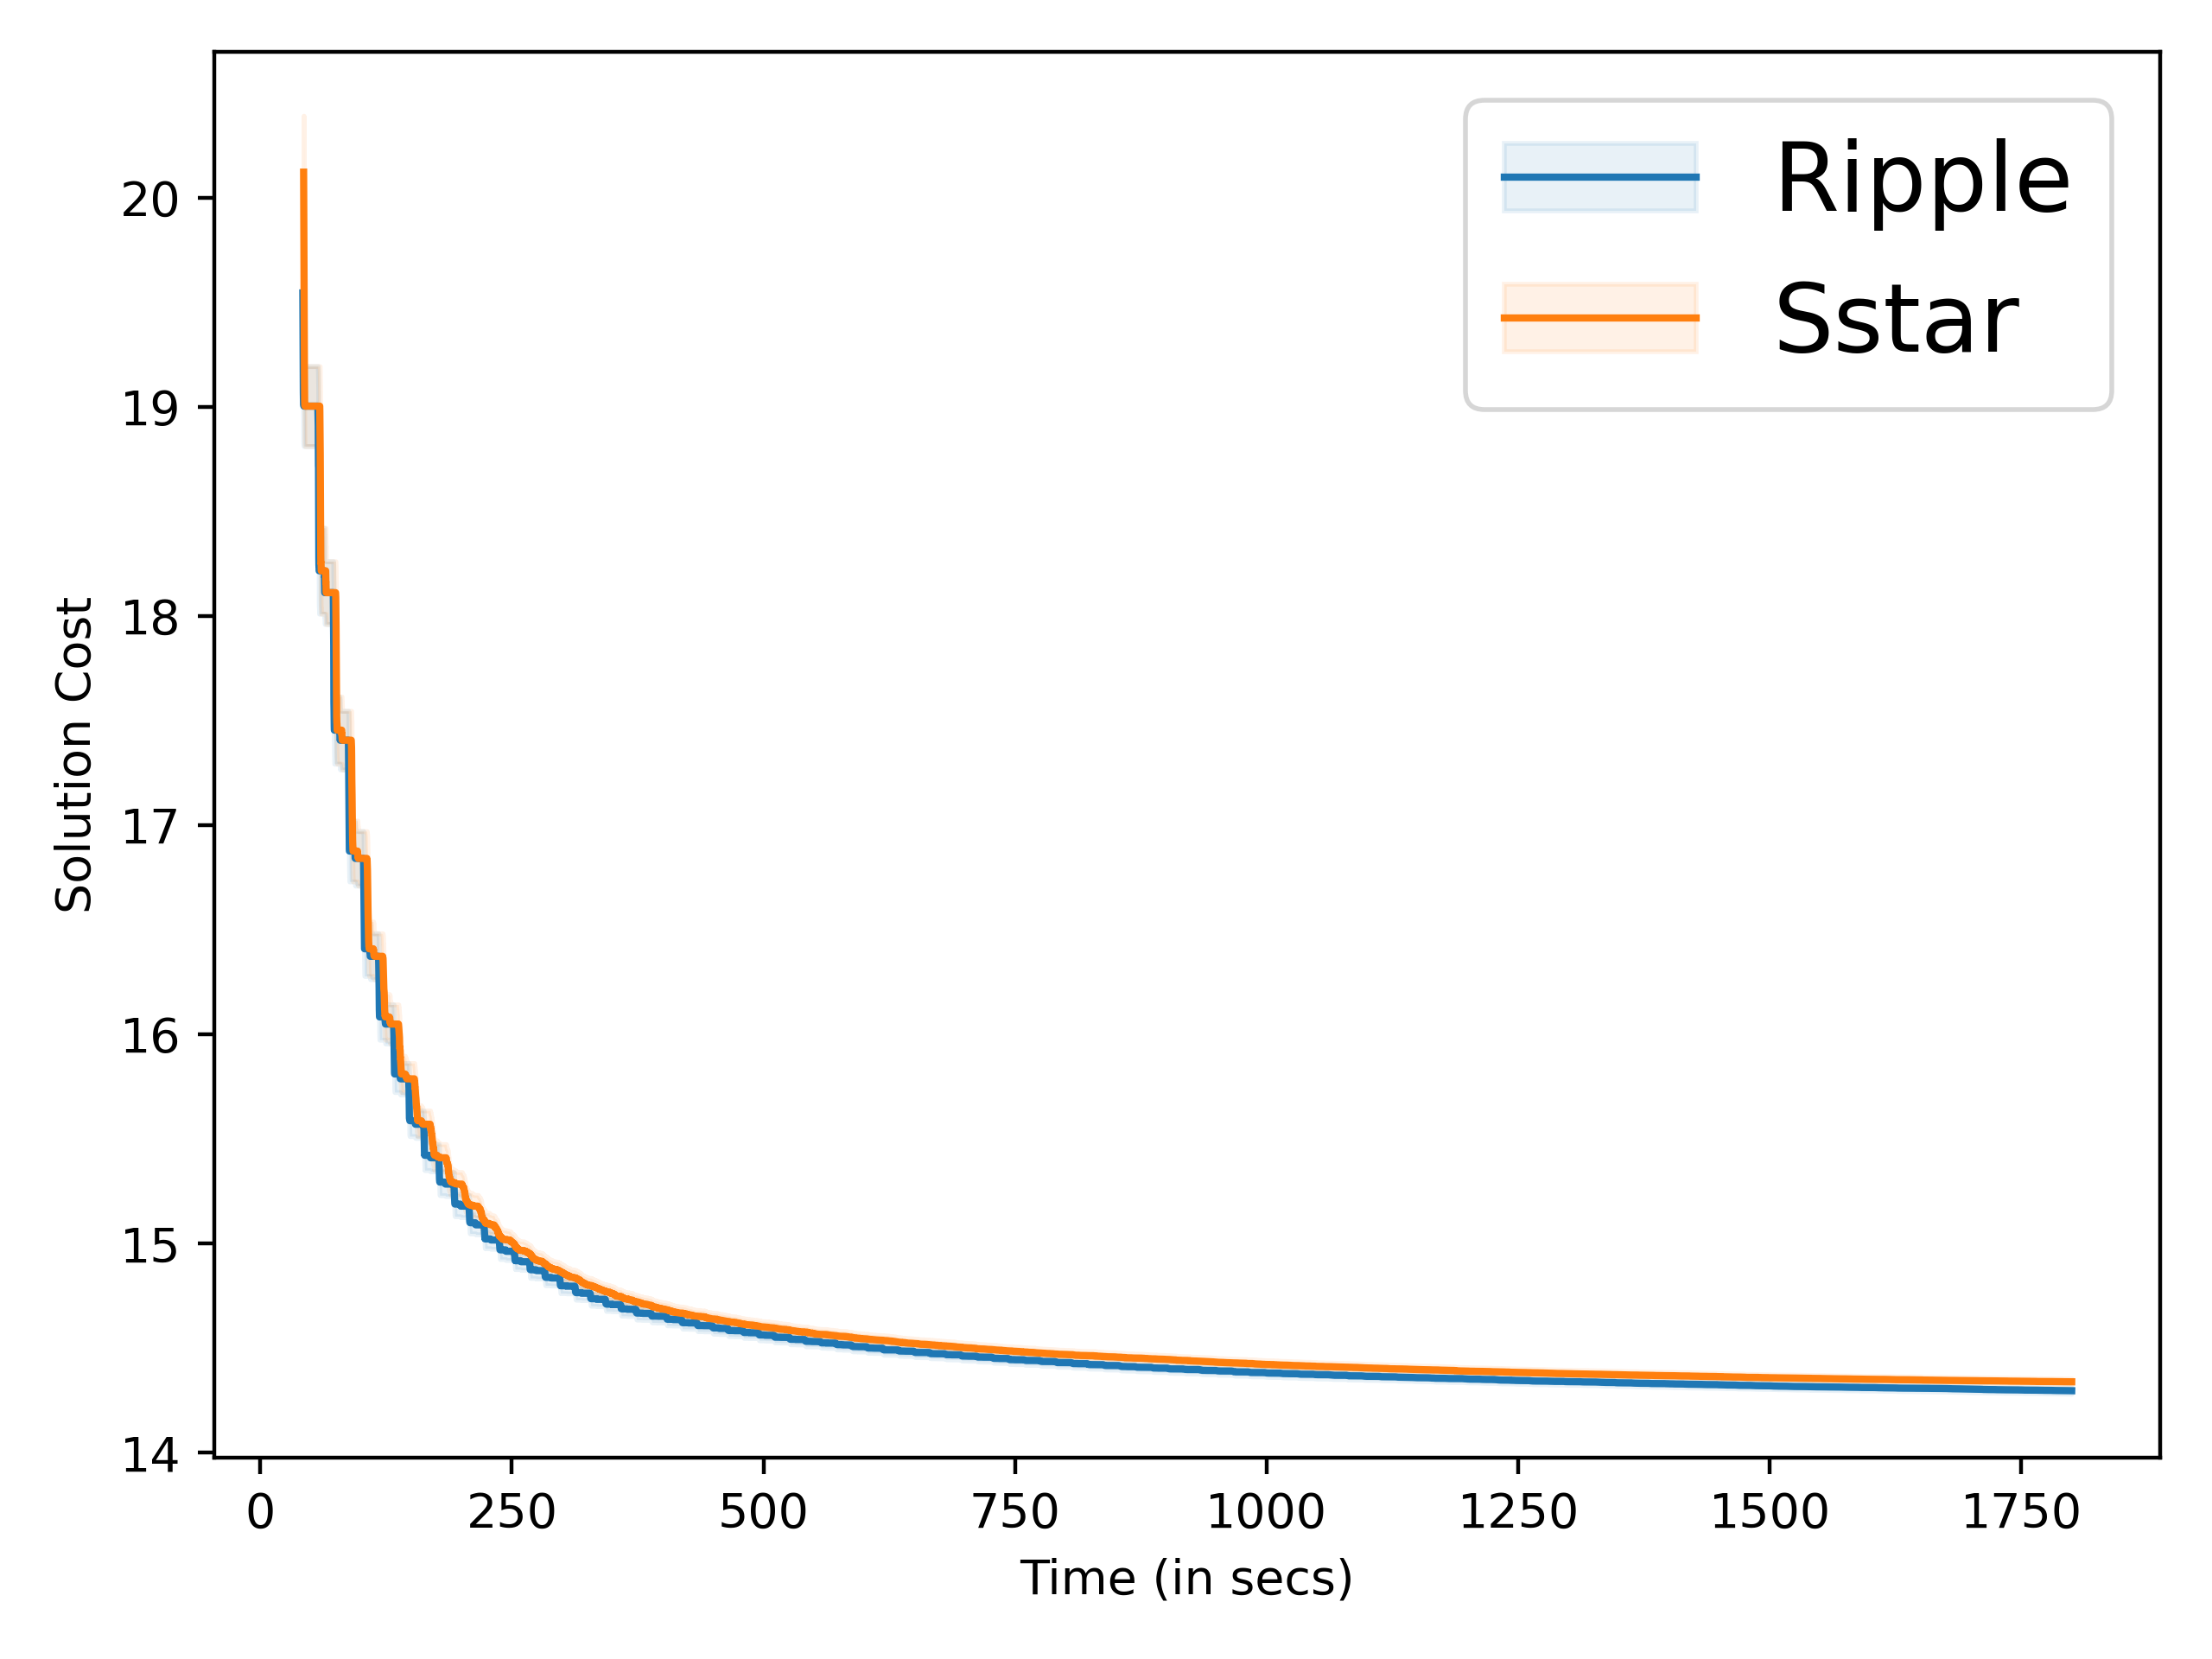} \\

   \makecell{\texttt{CO} \\ $\mathbb{R}^4$} & 
  \includegraphics[width=\linewidth, height=40mm]{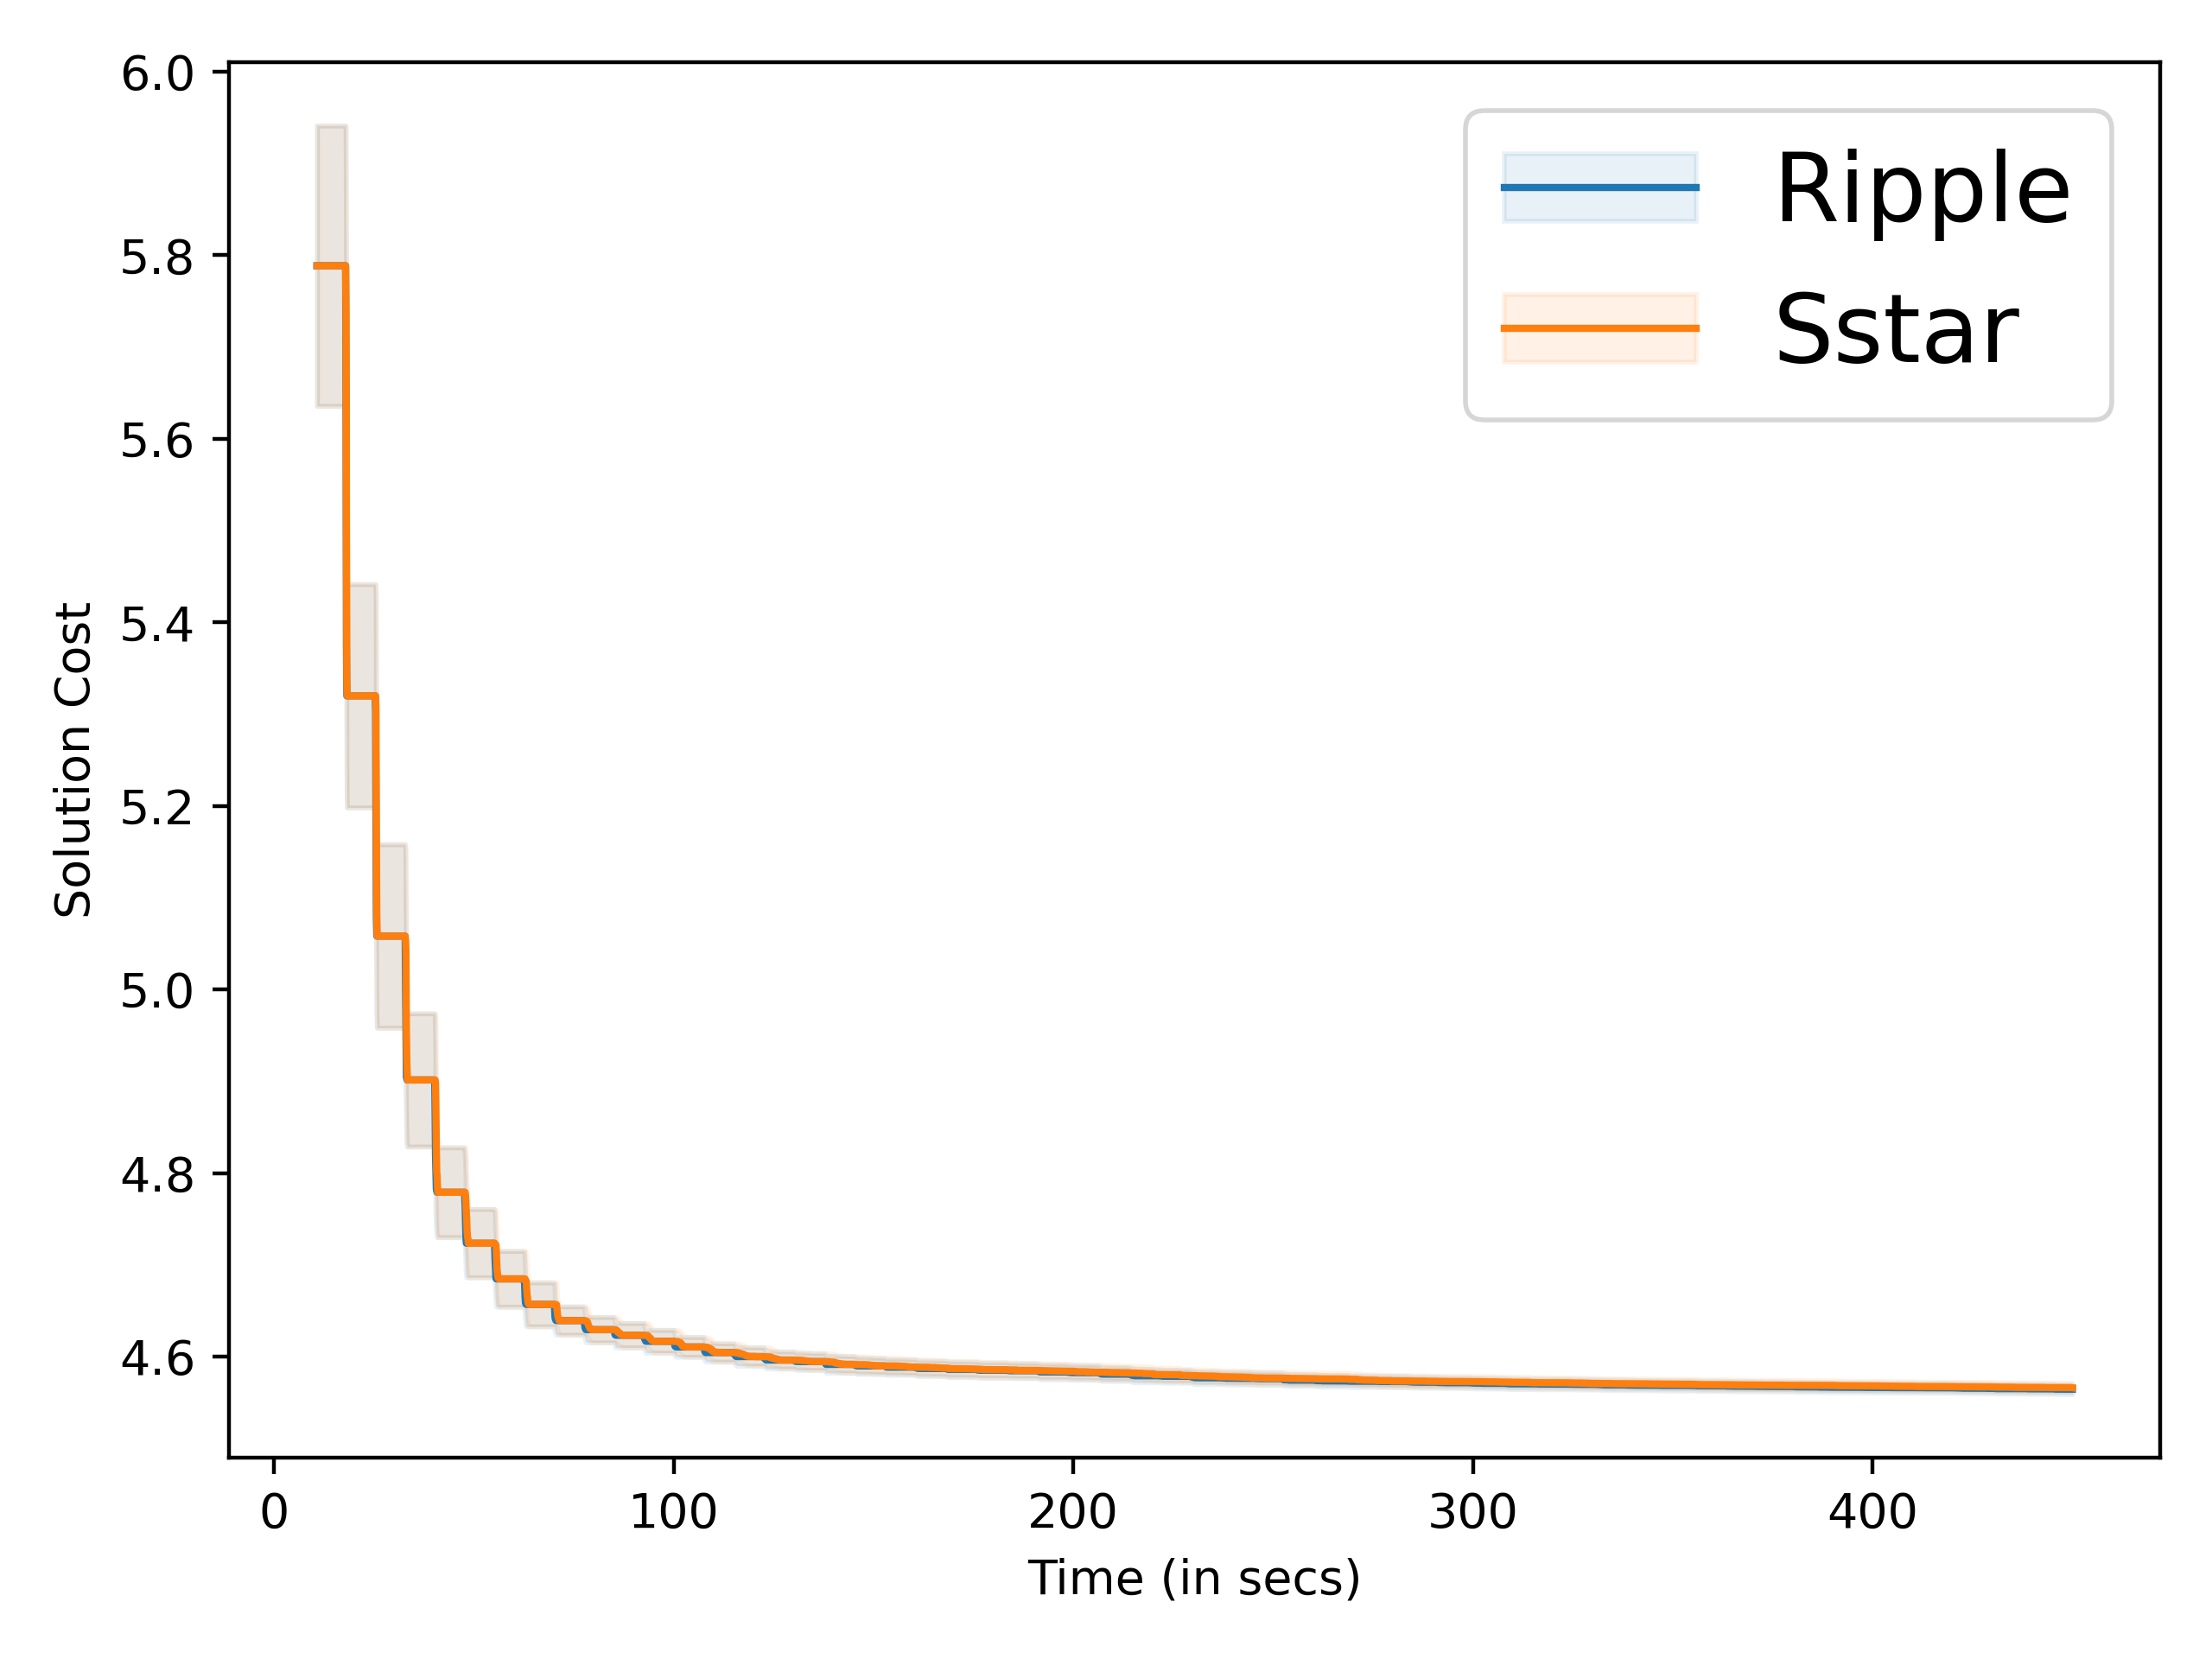}
   & \includegraphics[width=\linewidth, height=40mm]{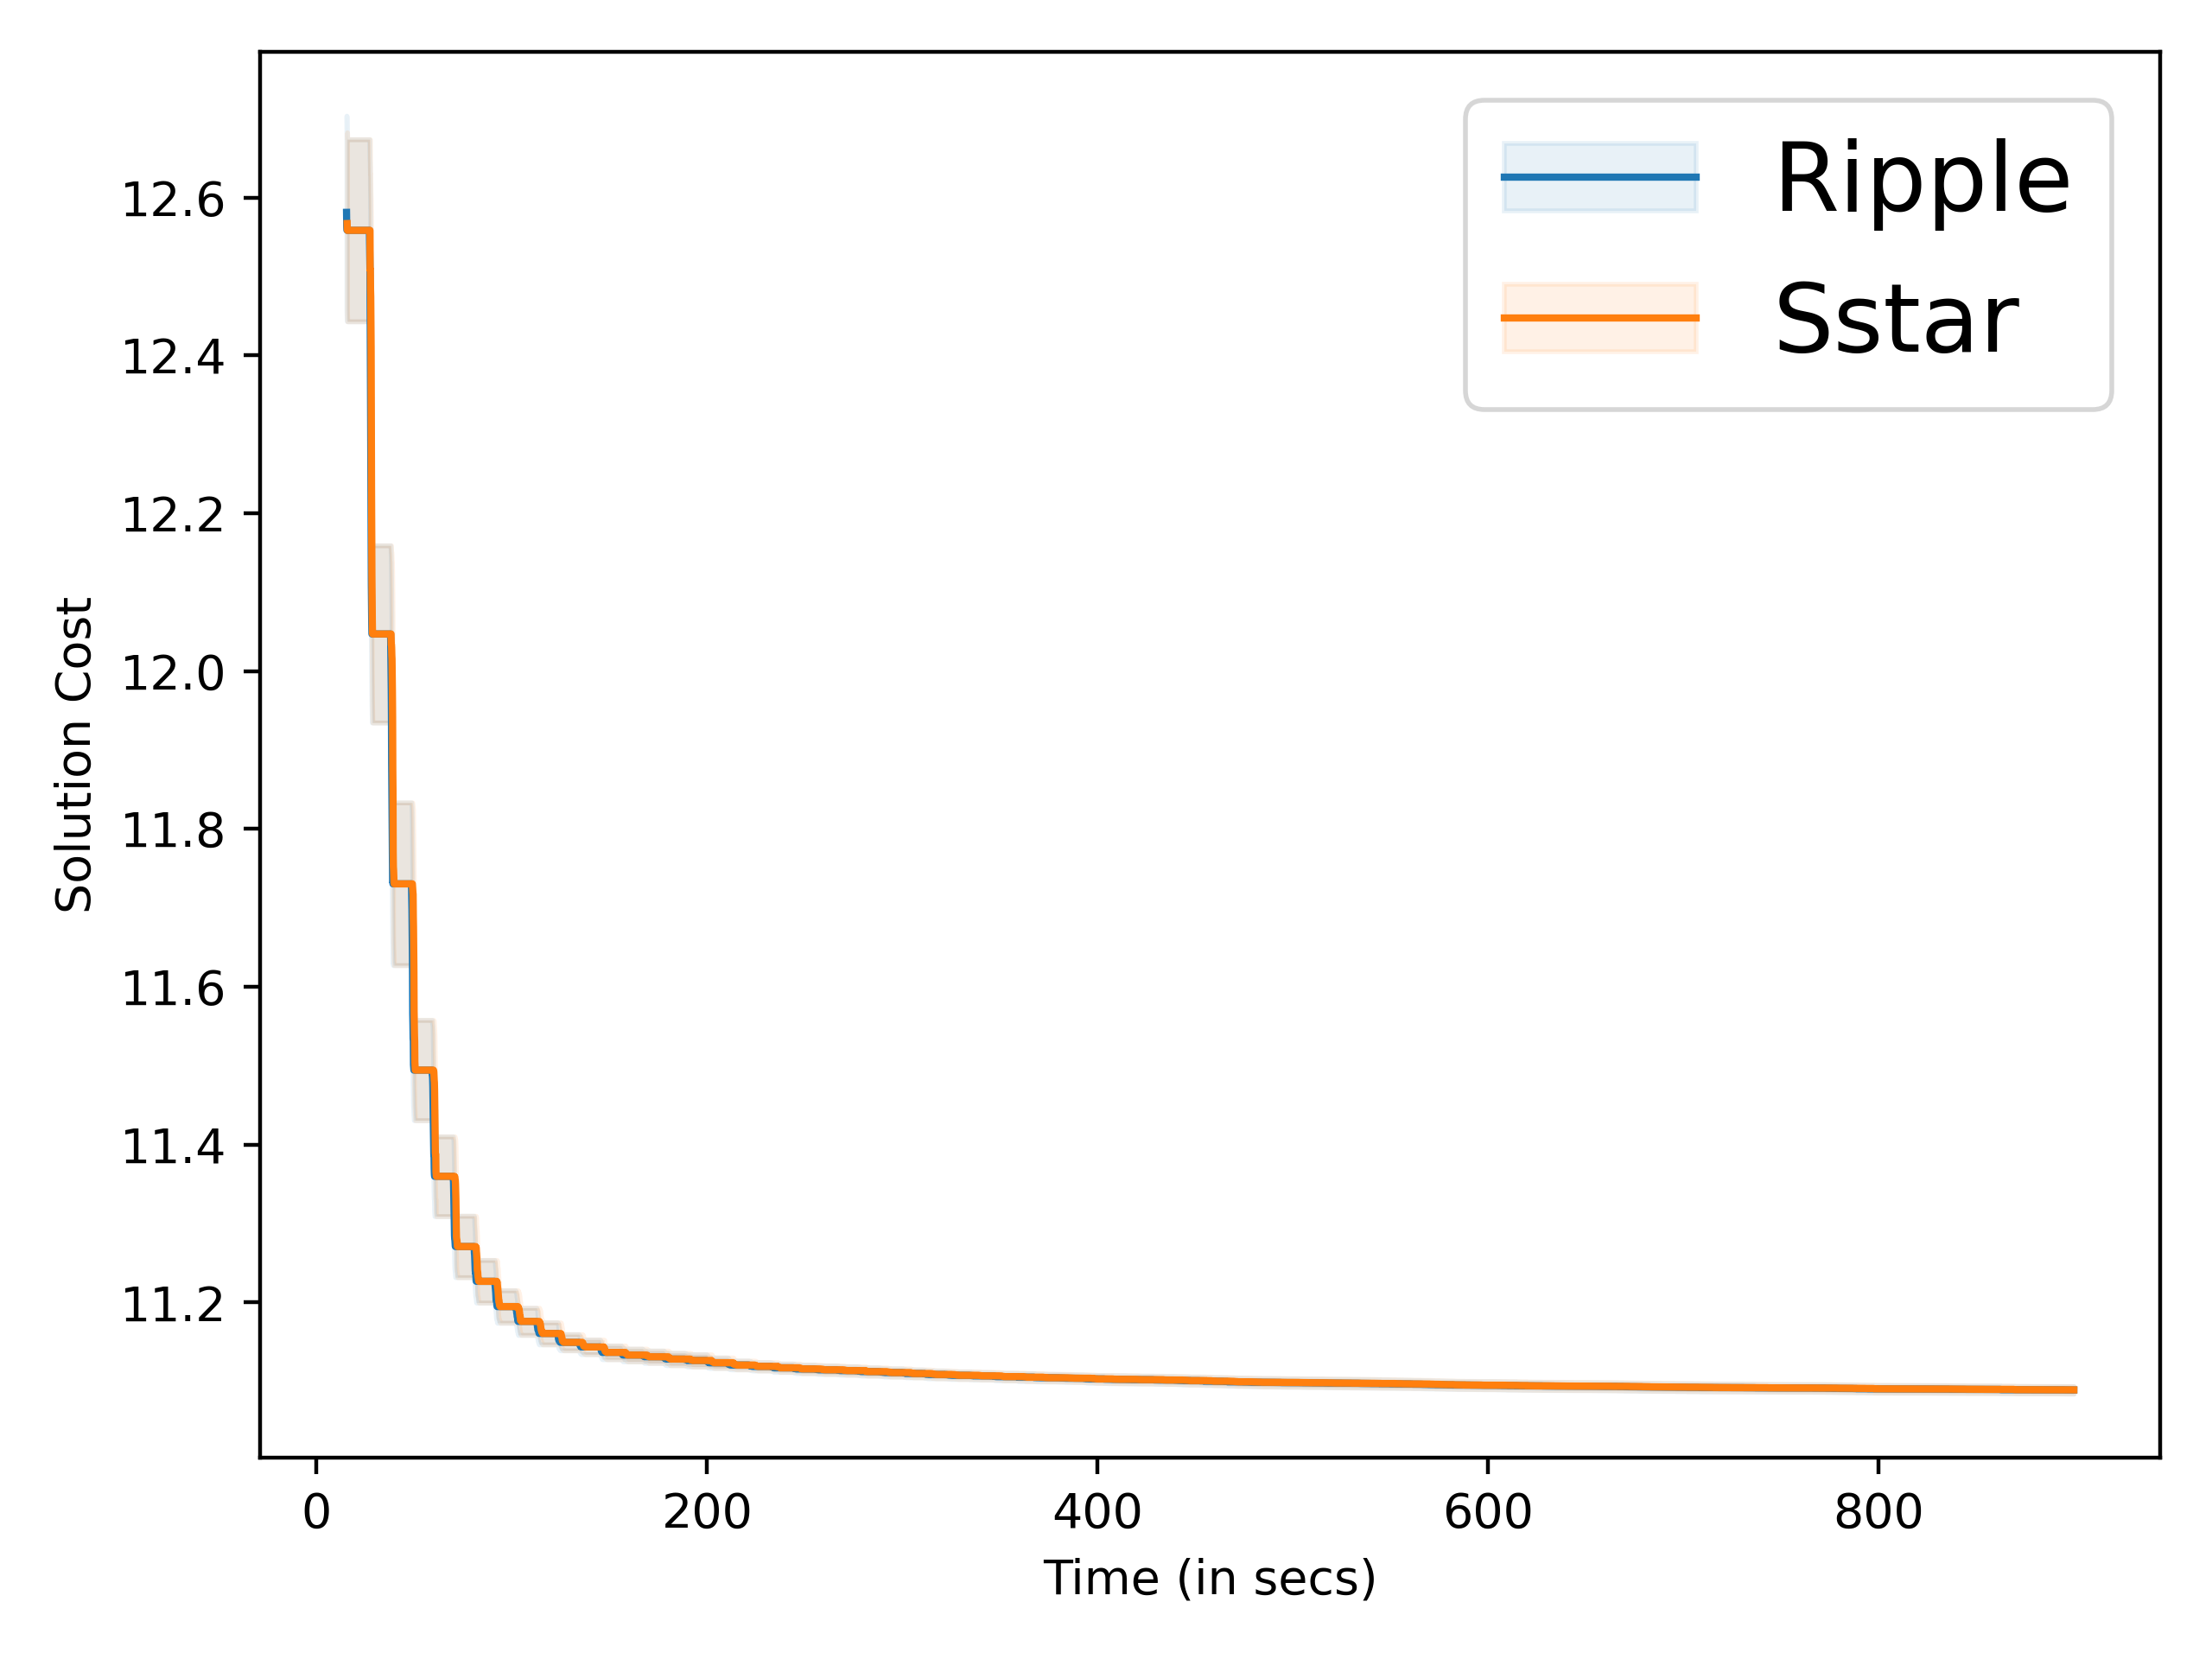} & \includegraphics[width=\linewidth, height=40mm]{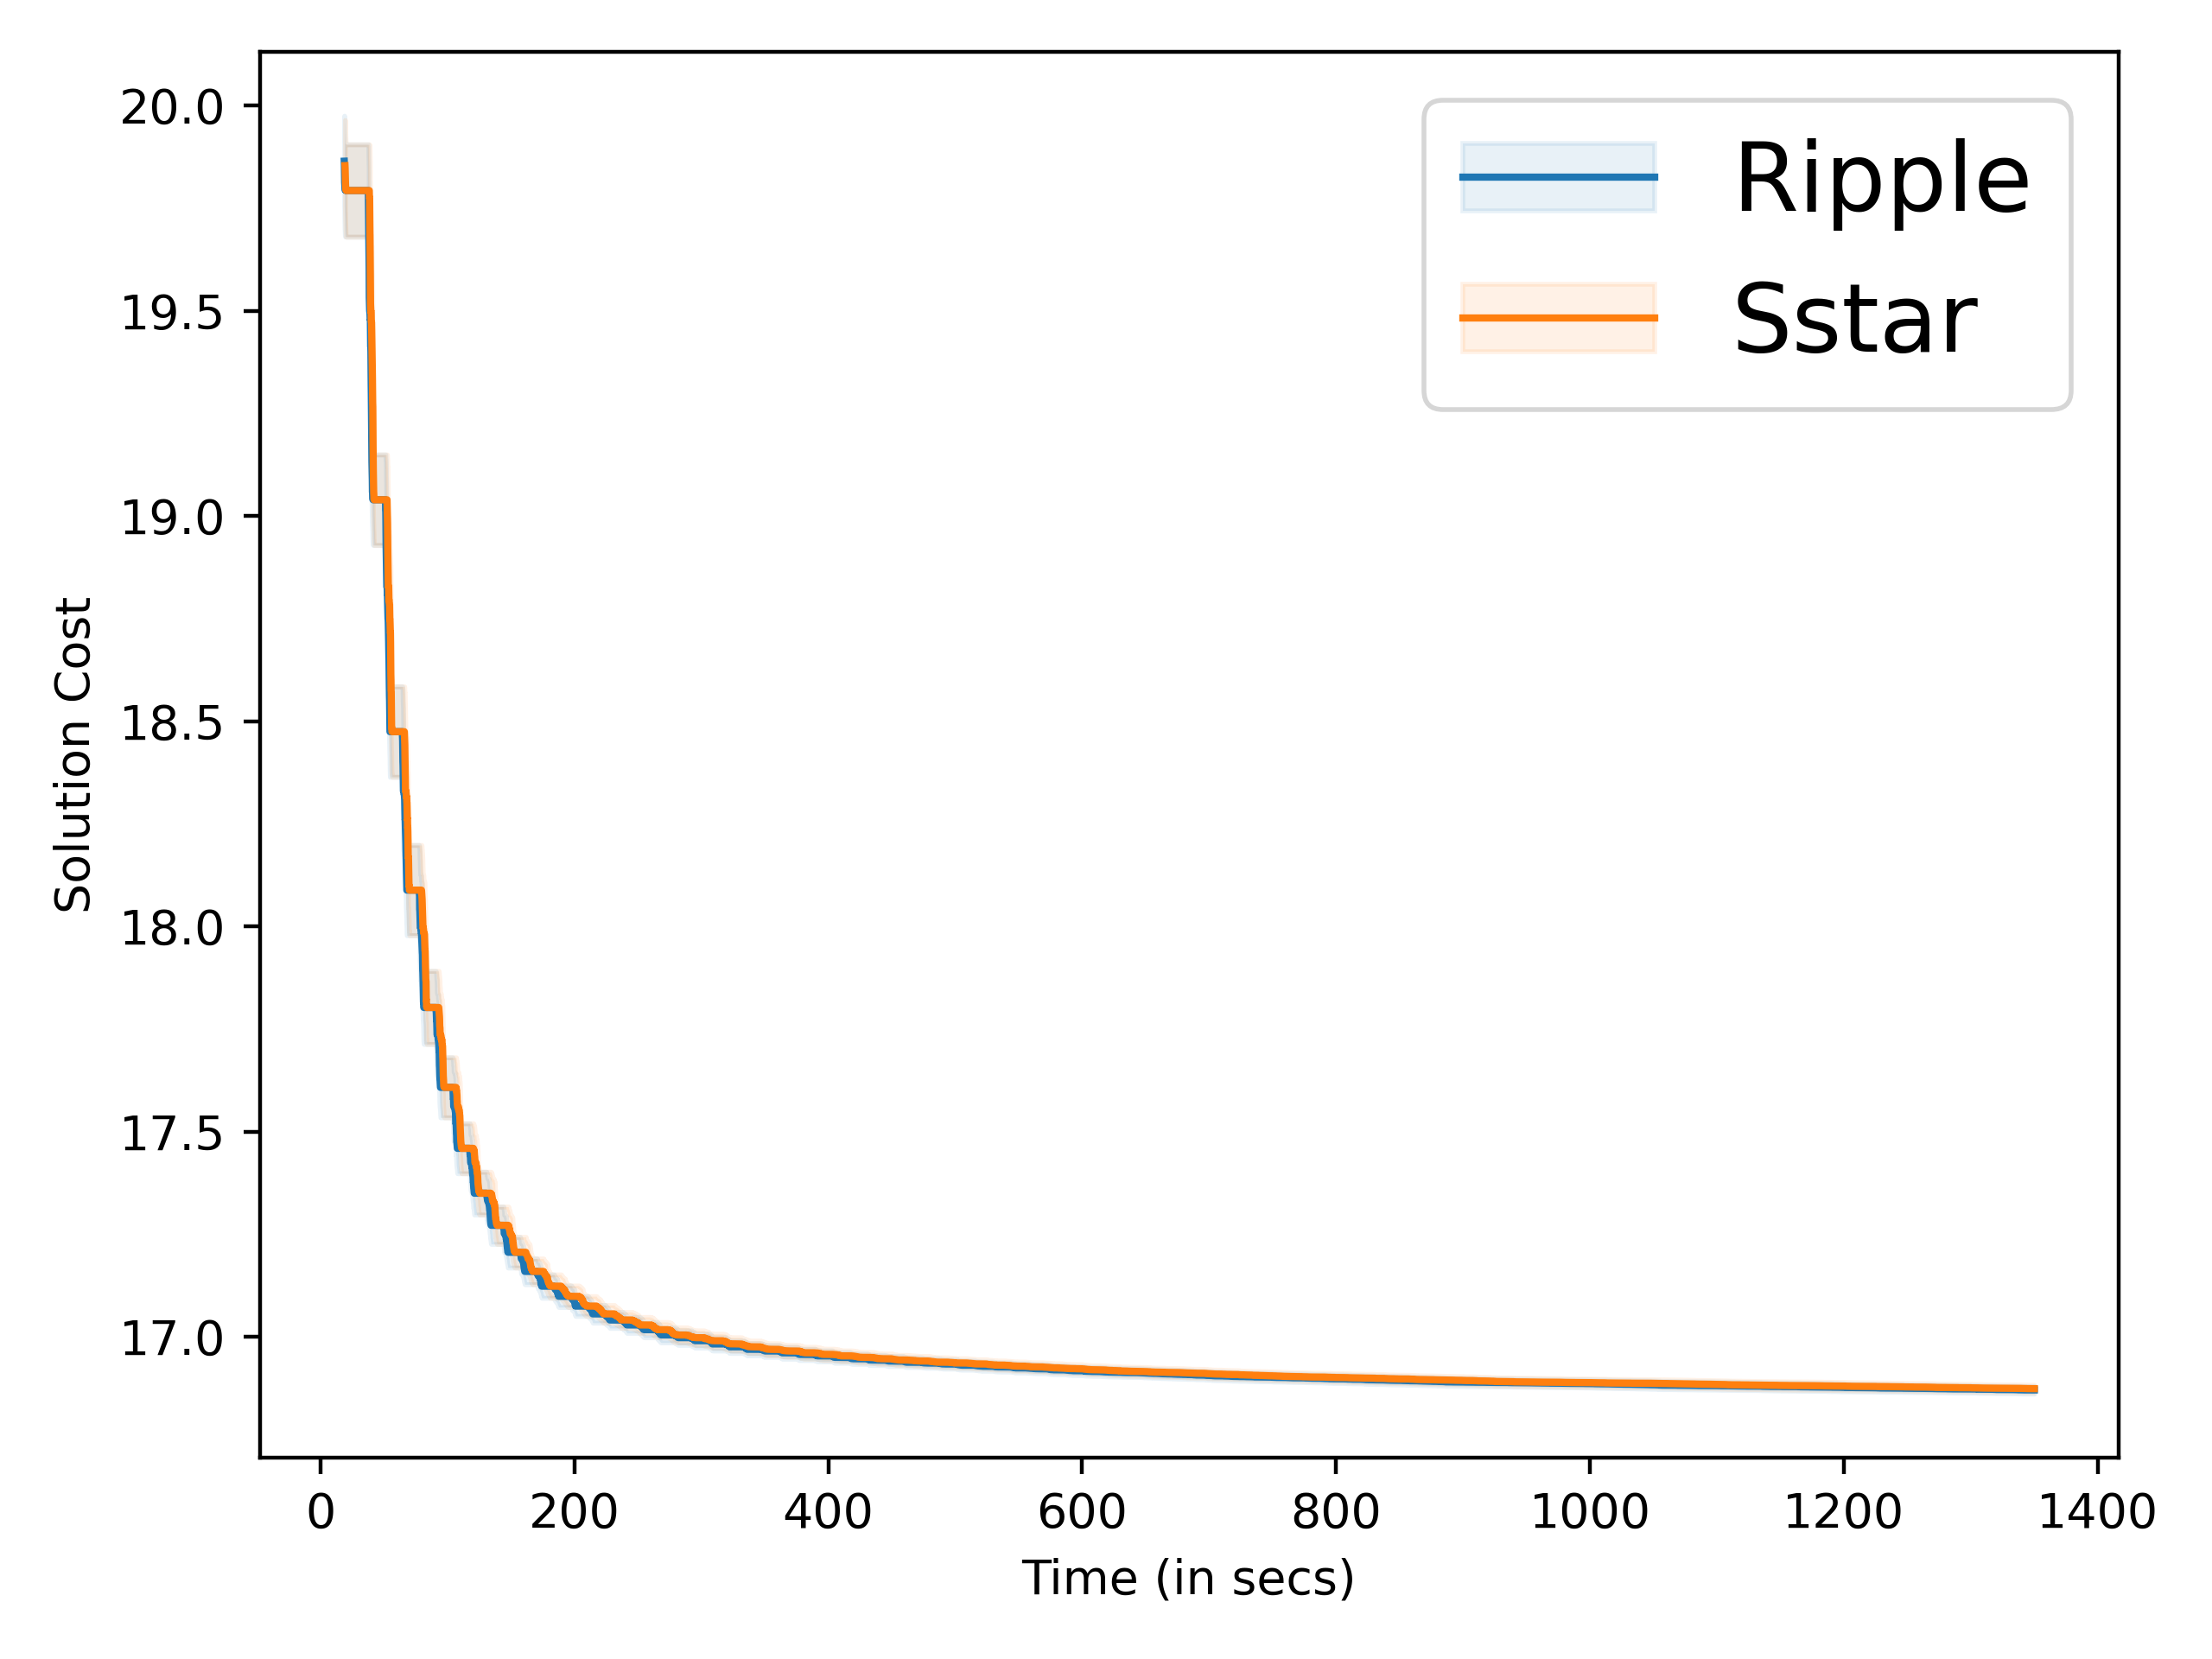} \\

   \makecell{\texttt{CO} \\ $\mathbb{R}^8$} & 
  \includegraphics[width=\linewidth, height=40mm]{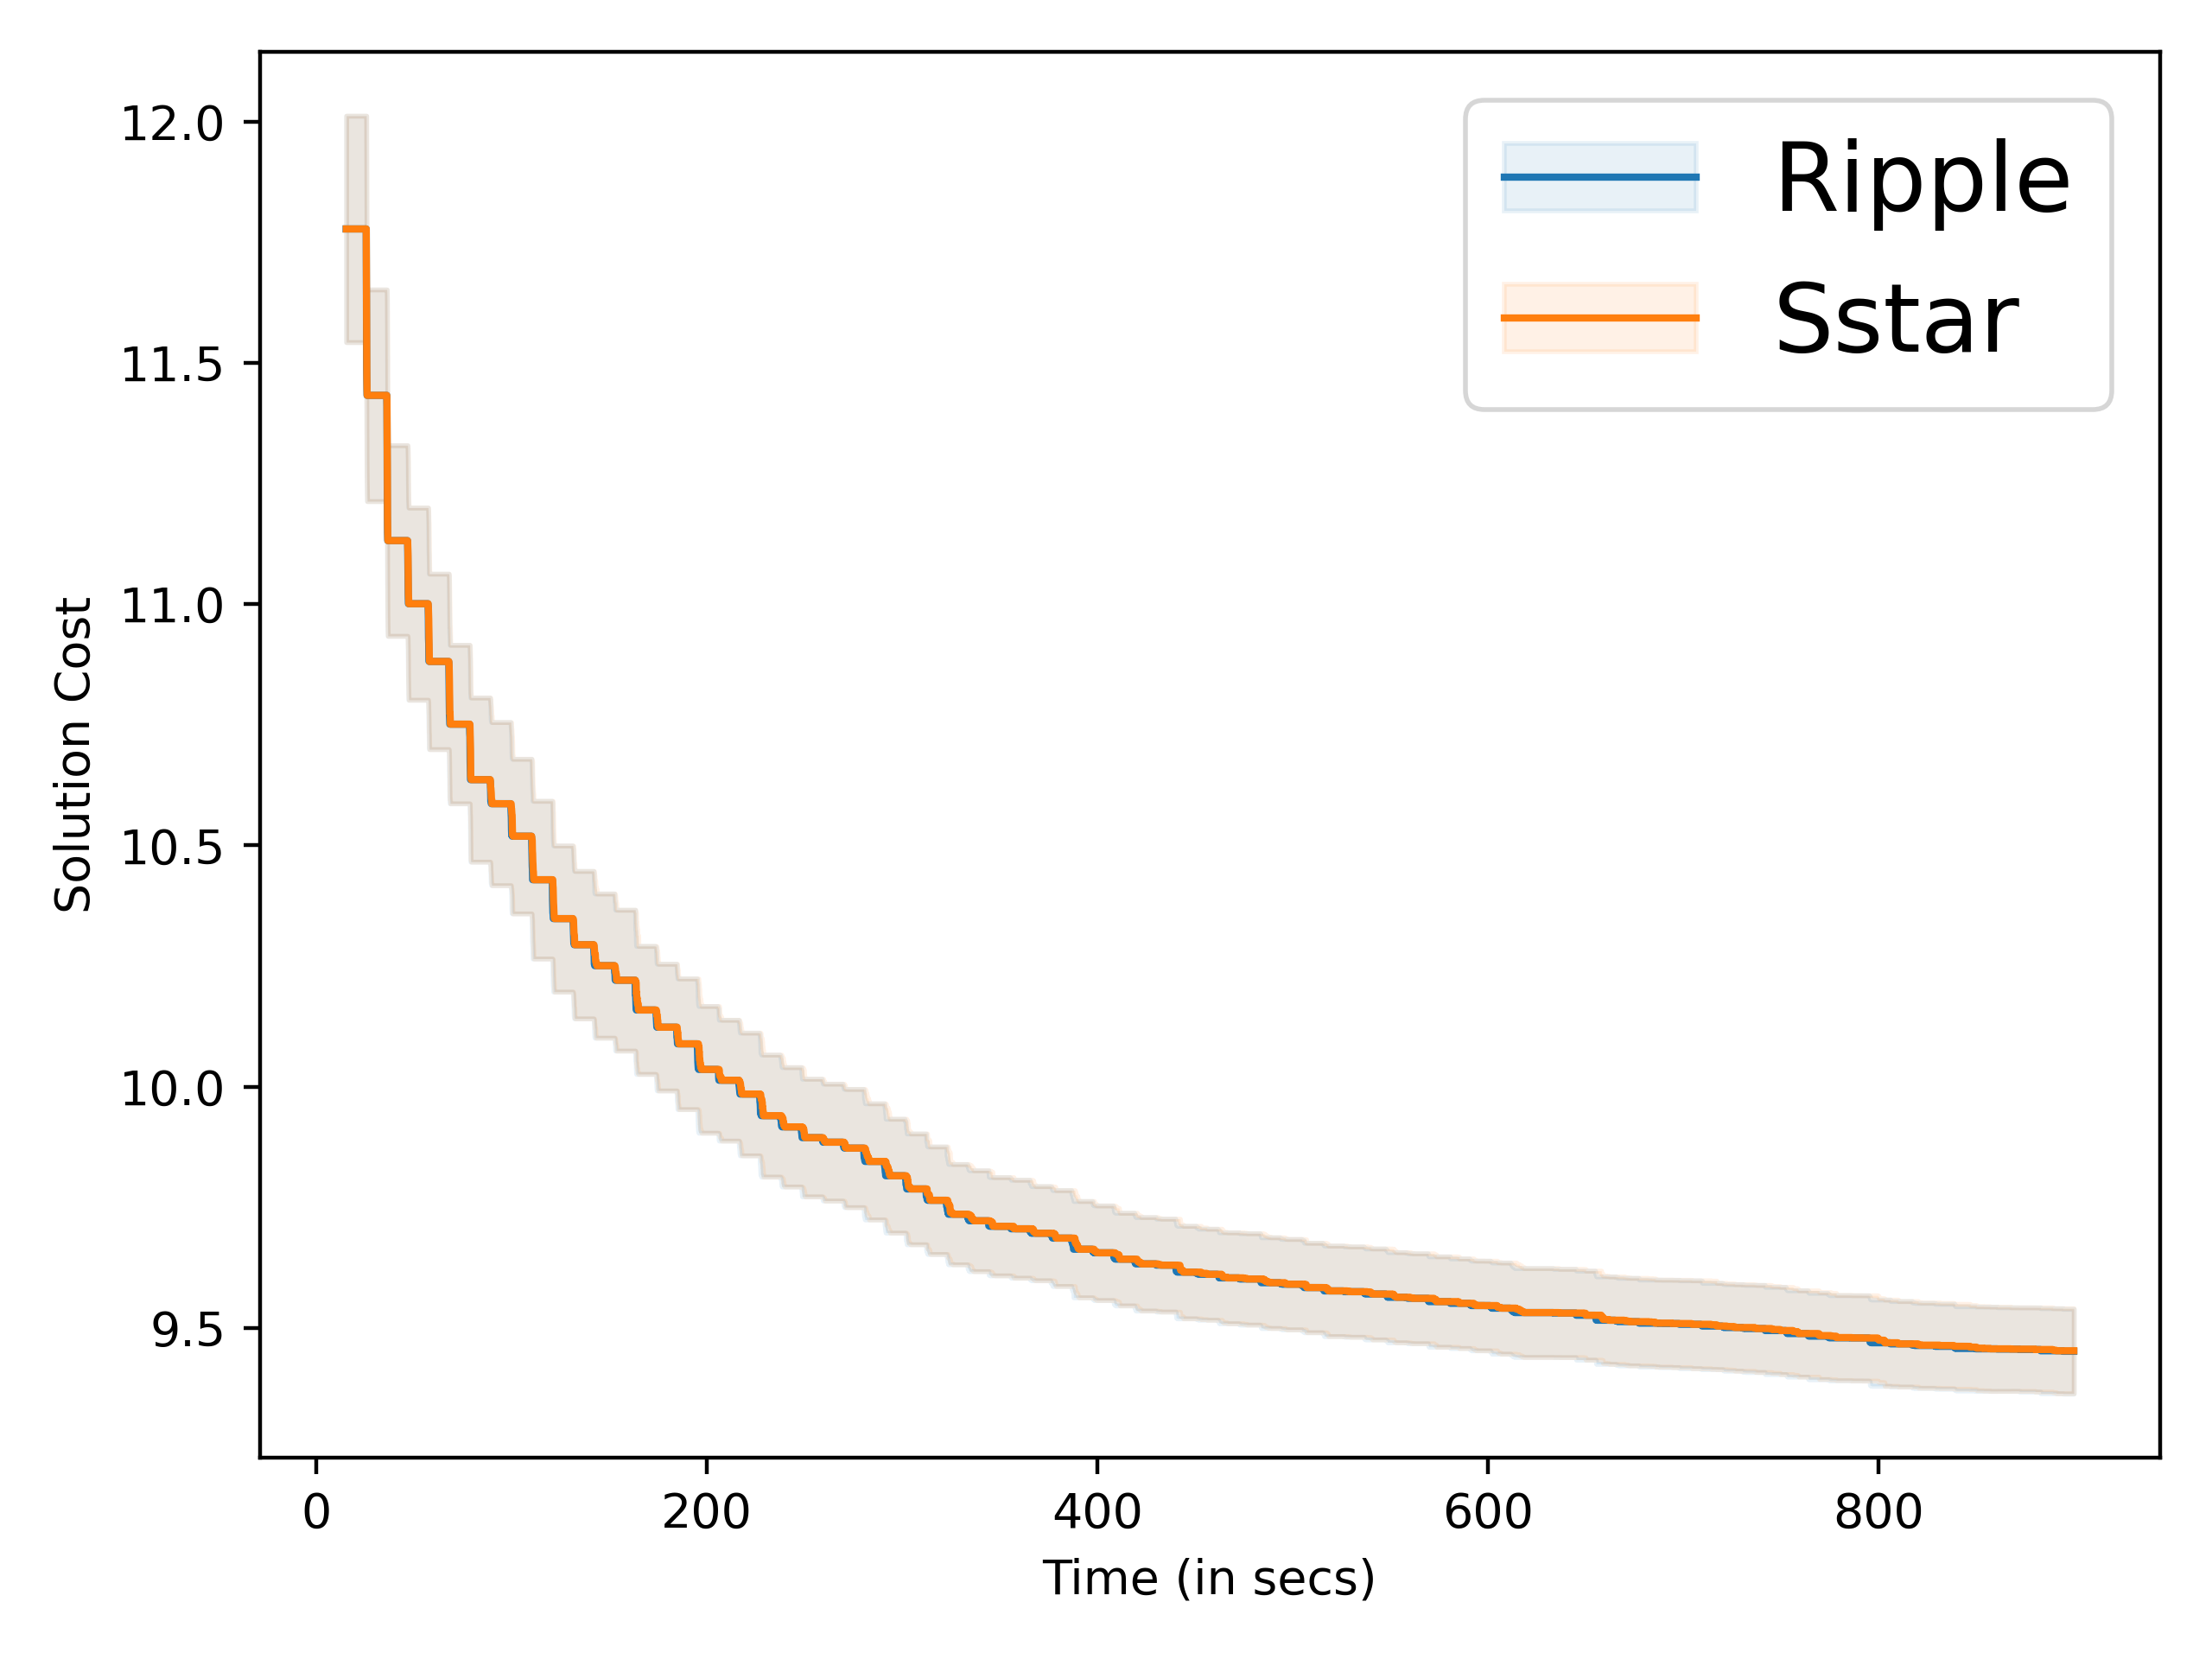}
   & \includegraphics[width=\linewidth, height=40mm]{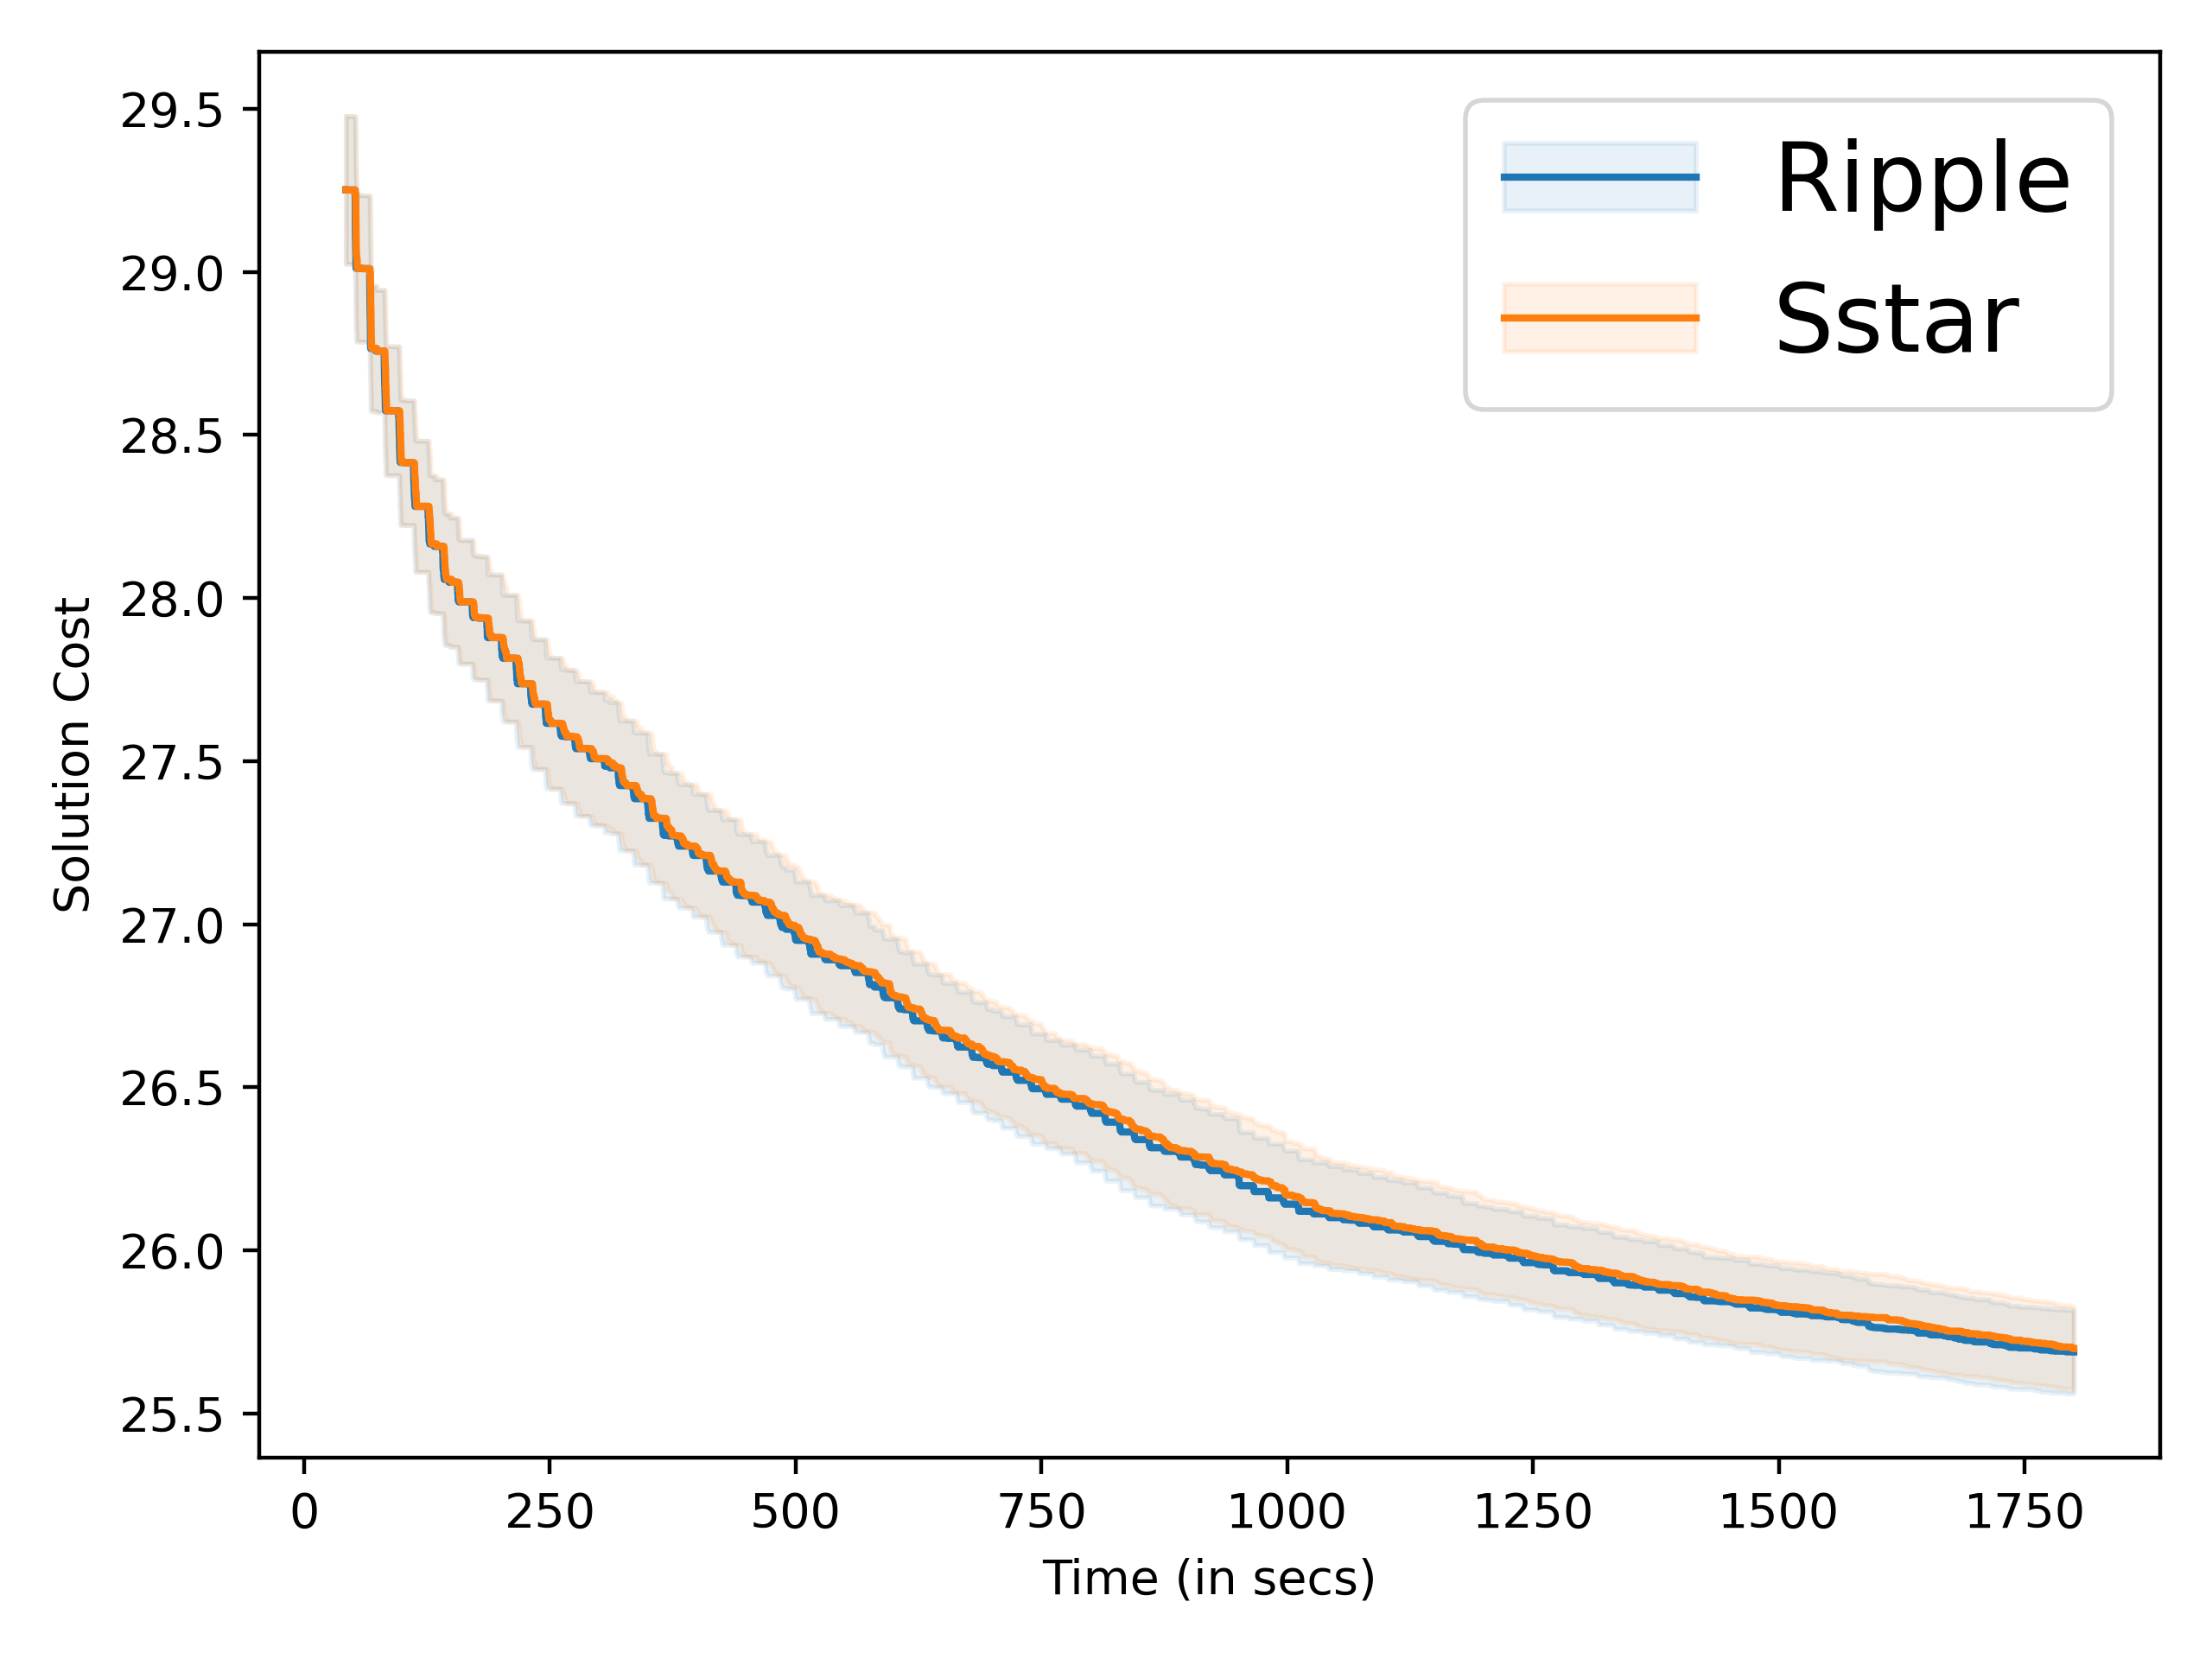} & \includegraphics[width=\linewidth, height=40mm]{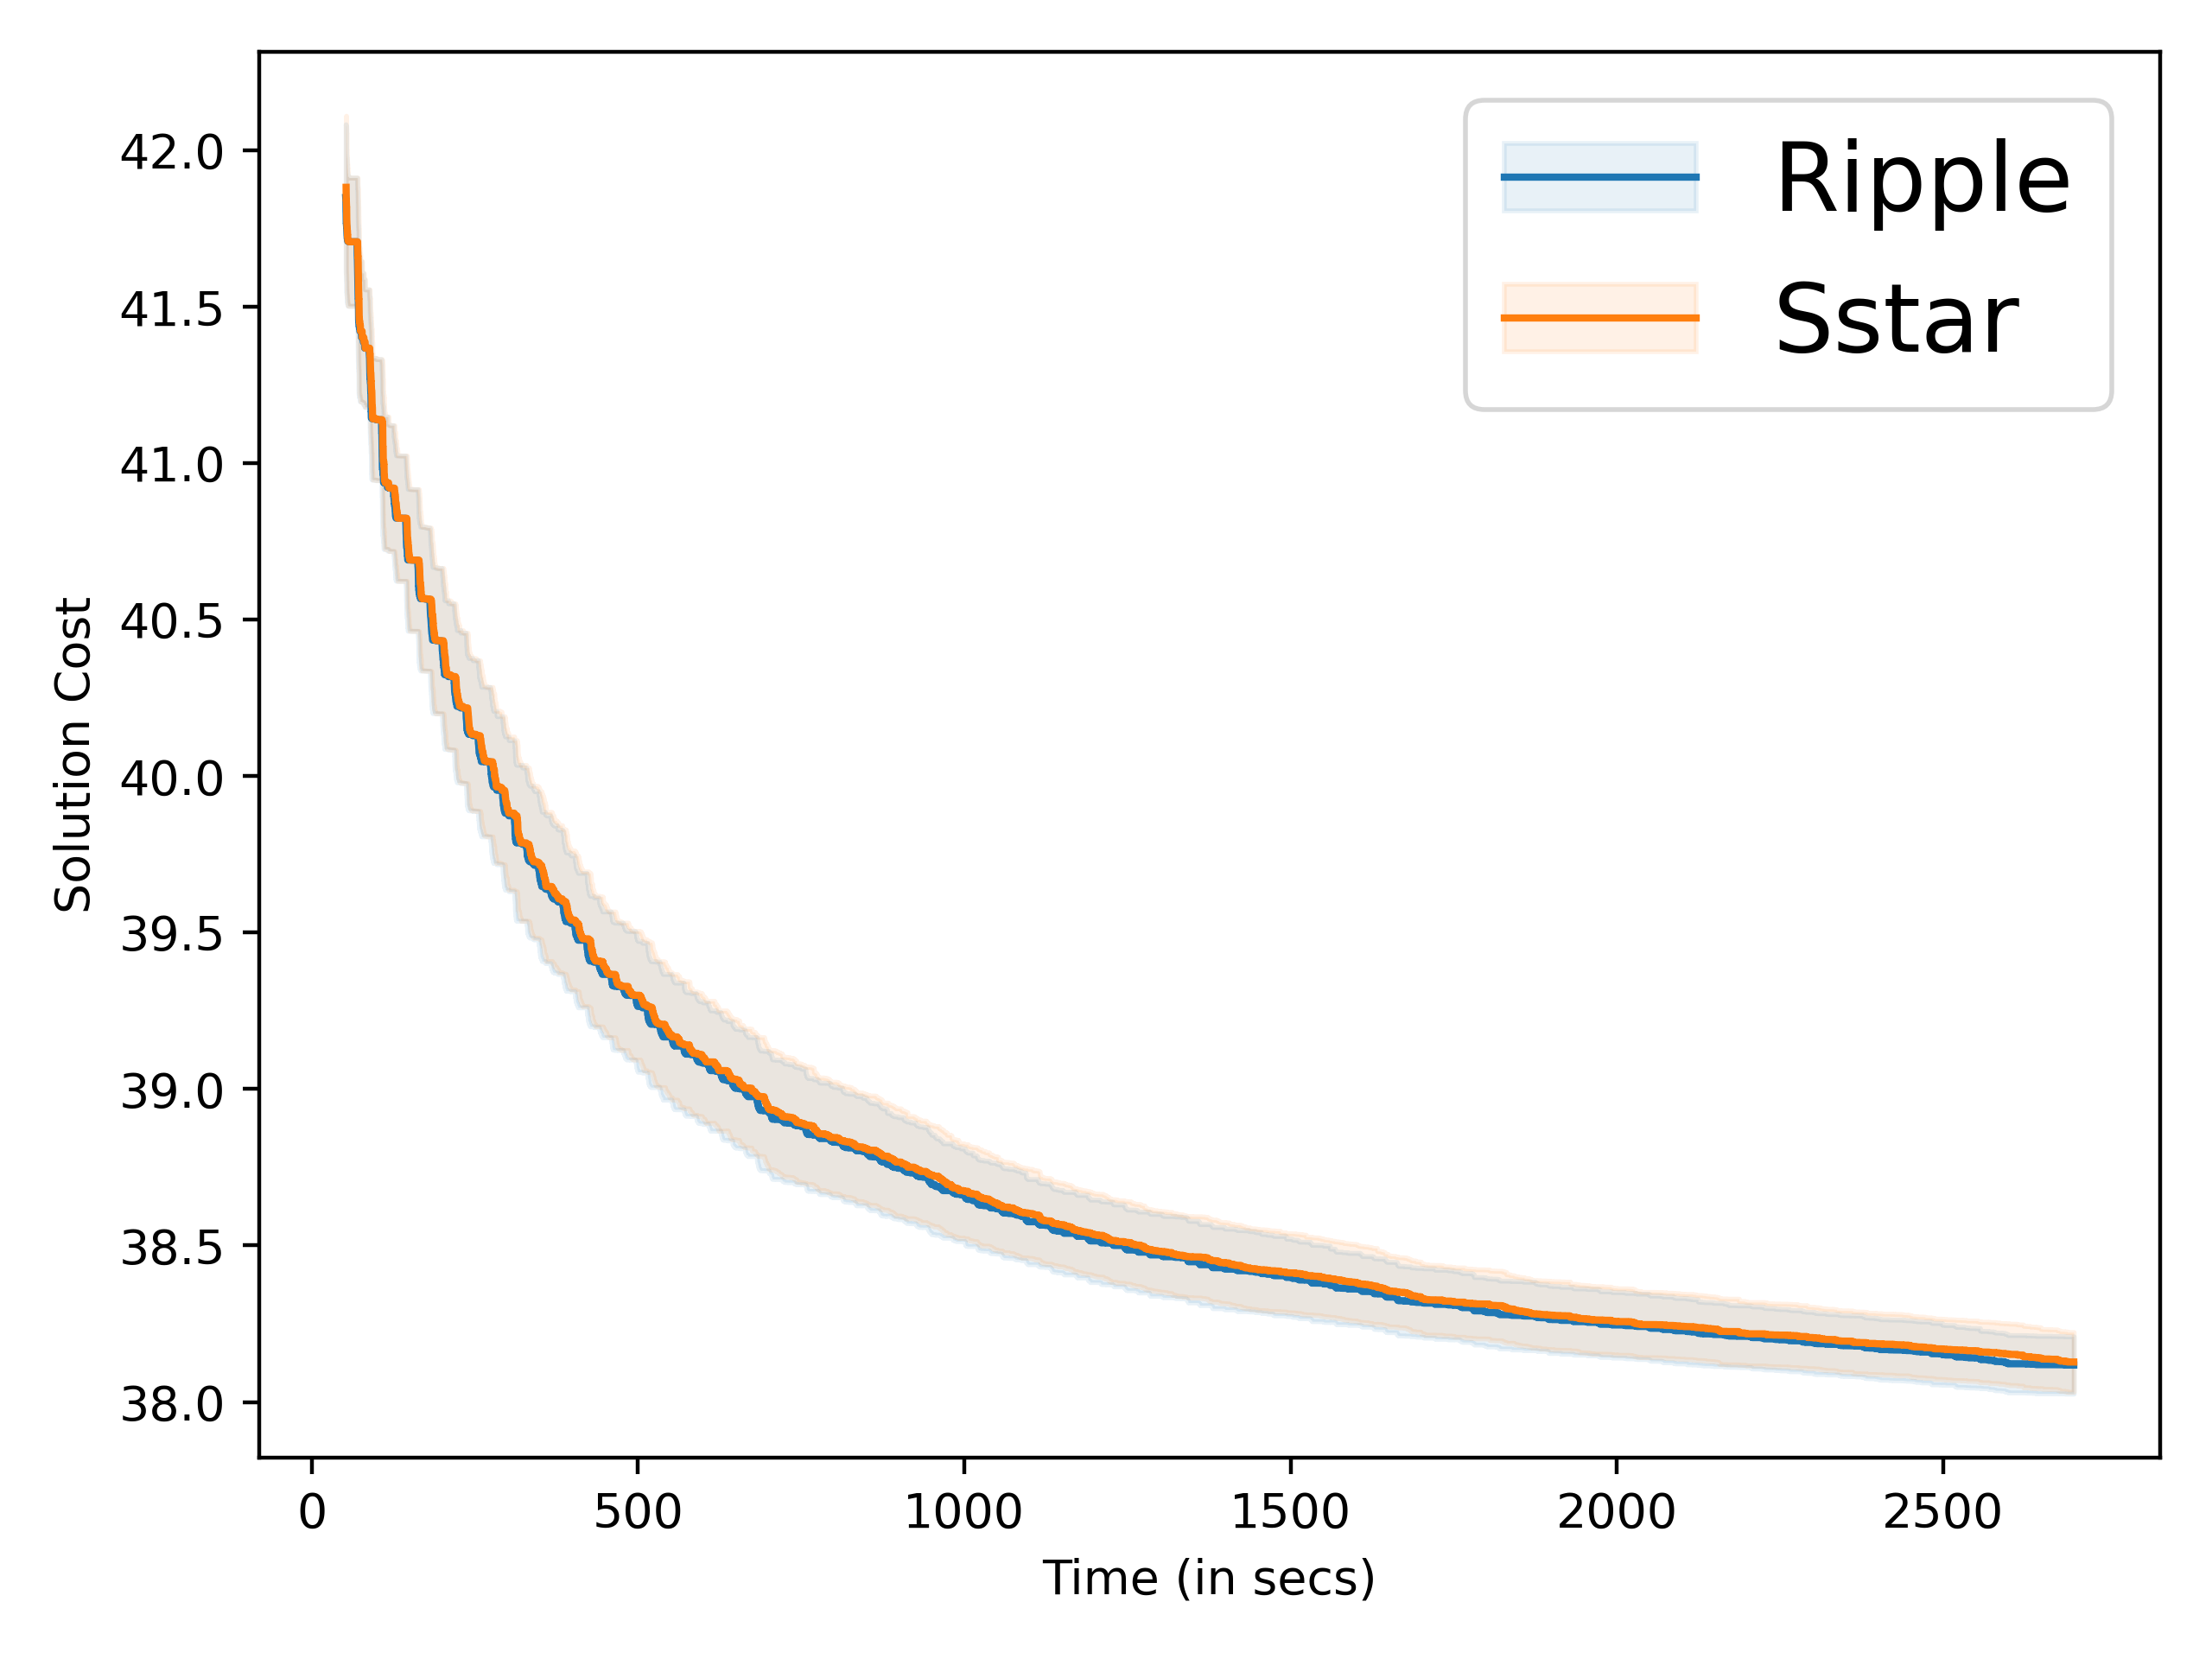} \\
   
            \bottomrule
            
        \end{tabular}
        \caption{Comparison of the performance of {IST\textsuperscript{*}} when {\alg Ripple} is used against S* on environments not shown in the main paper. The dark line represents the mean solution cost with the thick region being the 99\% confidence interval about the mean.}

        \label{tbl:RippleAppendix}
    \end{table*}

% \fi 
